# Supplementary material for: Iron: Intent-Aligned and Retrospective Dual Learning Framework for Enhancing Generalist Virtual Agents
Source: arXiv:2608.27866 source file (2026-08-28)
Supplement: Supplementary file 1 [file X_suppl.tex]

\clearpage

% --- 标题页 ---
\maketitlesupplementary



% --- 目录紧接在标题下方 (双栏模式) ---
% 在双栏下，我们使用 \small 或 \footnotesize 字体让目录更紧凑
\begin{center}
    \textbf{\large Table of Contents} % 保持 \large 字体，因为在双栏里 \Huge 会很大
\end{center}
\vspace{0.5em}

\begingroup
\renewcommand{\arraystretch}{1.2} 
\small % 使用 \small 字体，让目录内容更紧凑
% 关键修改：使用 l|r| 这种形式，让表格总宽度由内容决定并居中
% 或者使用 X 列，让 tabularx 自动居中。这里我们用定宽 p{...} 配合居中。
\begin{tabular}{p{0.8\columnwidth}r} % <<--- 关键：宽度从 0.9 减小到 0.8，并确保表格能居中
    \textbf{A Details of Imitation Learning} \dotfill & 1 \\
    \quad A.1 Unified Action Space \dotfill & 1 \\
    \quad A.2 Intent Understanding Data Collection \dotfill & 1 \\
    \quad A.3 Training Details \dotfill & 2 \\
    \quad A.4 Prompt Details \dotfill & 2 \\
    \textbf{B The MCTS Algorithm and Hyperparameters} \dotfill & 2 \\
    \quad B.1 Algorithmic Workflow \dotfill & 2 \\
    \quad B.2 Selection of Node Count \dotfill & 3 \\
    \quad B.3 Maximum Search Tree Depth \dotfill & 3 \\
    \quad B.4 Analysis of MCTS Efficiency and Data Generation Cost \dotfill & 3 \\
    
    \textbf{C Stepwise Cycle-Consistent Reward Details} \dotfill & 4 \\
    \quad C.1 Prompt for Calculating the Matching Score \dotfill & 4 \\
    \quad C.2 Example of Stepwise Cycle-Consistent Reward \dotfill & 4 \\
    \quad C.3 SCC Reward Analysis \dotfill & 5 \\
    \textbf{D Supplementary Procedures for Hindsight Reproduction and Trajectory Filtering} \dotfill & 5 \\
    \quad D.1 Self-Prompting Mechanism \dotfill & 5 \\
    \quad D.2 Trajectory Filtering Metrics \dotfill & 5 \\
    \quad D.3 Filtering Calculate Method \dotfill & 6 \\
    \quad D.4 Semantic Accuracy Analysis of Hindsight Reproduction \dotfill & 6 \\
    \textbf{E Details of Self-training} \dotfill & 7 \\
    \quad E.1 Training Details \dotfill & 7 \\
    \quad E.2 Impact of Iterative Training \dotfill & 7 \\
    \textbf{F Evaluation Details} \dotfill & 7 \\
    \quad F.1 Benchmarks \dotfill & 7 \\
    \quad F.2 Baselines\dotfill & 7 \\
    \quad F.3 Statistical Significance Analysis \dotfill & 8 \\
    \quad F.4 A successful task completion example \dotfill & 9 \\
\end{tabular}
\endgroup

% --- 附录主体内容紧接其后 ---
% 不需要 \newpage，内容会紧接着目录在同一栏或下一栏继续。
\pagestyle{plain}
% \twocolumn 已经在上面启动


\section*{A\ \ \ Details of Imitation Learning}\label{app:A}
This section details the implementation of our imitation learning-based \textbf{\textit{Iron}} framework. We begin by defining the unified action space that enables our agent to operate across diverse digital environments. Following this, we outline the full training procedure, including the methodology for collecting intent understanding data. Finally, we provide a complete list of the system and user prompts that unify our agent's four core capabilities: task planning, intent understanding, element grounding, and state description, into a single, robust framework.

\subsection*{A.1\ \ \ Unified Action Space}


In this section, we introduce \textit{\textbf{Iron}}'s unified action space. This design adopts Aguvis's core philosophy, combining standard PyAutoGUI actions with unique context-aware actions to ensure the agent model's generality across environments and flexibility in specific environments. This allows the model to seamlessly adapt to various operating systems and application scenarios while enabling more precise and detailed interactions.

\begin{table}[htbp]
    \centering
    \caption{Core PyAutoGUI Actions in Iron's Framework}
    \label{tab:core_actions}
    \footnotesize
    \begin{tabularx}{\linewidth}{lX}
        \toprule
        \textbf{Category} & \textbf{Action Space} \\
        \midrule
        \textbf{Fundamental} & \texttt{pyautogui.moveTo(point\_x, point\_y)} \\
                              & \texttt{pyautogui.click(point\_x, point\_y)} \\
                              & \texttt{pyautogui.write('text\_to\_type')} \\
                              & \texttt{pyautogui.press('key\_identifier')} \\
                              & \texttt{pyautogui.hotkey('ctrl', 'v')} \\
                              & \texttt{pyautogui.scroll(-100)} \\
                              & \texttt{pyautogui.dragTo(final\_x\_coord, final\_y\_coord)} \\
        \bottomrule
    \end{tabularx}
\end{table}

% --- 第二个表格：可插拔动作 (已根据您的要求修改) ---
\begin{table}[htbp]
    \centering
    \caption{Extended Pluggable Actions for Specific Contexts}
    \label{tab:pluggable_ext_actions_v2} % 更改标签以示区别
    \footnotesize % 字体保持不变
    \begin{tabularx}{\linewidth}{lX}
        \toprule
        \textbf{Category} & \textbf{Action Space} \\
        \midrule
        \textbf{Context-Aware} & \texttt{browser.select\_option (x, y, value)} \\ % 简化变量
                               & \texttt{mobile.swipe (from, to)} \\ % 简化变量
                               & \texttt{mobile.home()} \\
                               & \texttt{mobile.back()} \\
                               & \texttt{mobile.open\_app (name)} \\ % 简化变量
                               & \texttt{mobile.terminate (status)} \\ % 简化变量
                               & \texttt{answer (text)} \\ % 简化变量
        \dots & \dots \\ % 省略号移到这里
        \bottomrule
    \end{tabularx}
\end{table}
% 补充这里的内容
\subsection*{A.2\ \ \ Intent Understanding Data Collection}

We first utilized the Qwen2.5-VL-72B-Instruct  model to generate 20k intent understanding training data by randomly selecting images and operation sequences from the Aguvis  dataset; this data then distilled our initial model for \textit{intent understanding.}

Our prompt used for collecting intent understanding data is as follows:
\begin{tcolorbox}[
    % colback=gray!5!white, % 背景颜色已移除
    colframe=black, % 边框颜色设置为黑色
    title=\textbf{\textit{Intent Understanding Prompt}}, % 标题
    fonttitle=\bfseries\rmfamily, % 标题字体
    arc=2mm, % 圆角
    boxsep=1mm, % 边框与内容间距
    left=3mm, right=3mm, top=2mm, bottom=2mm, % 内部填充
    breakable=true, % 允许跨页断开
    sharp corners=west, % 例如：只有左侧为直角
    % width=\columnwidth, % 如果在双栏模式下希望宽度为单栏
    % width=\textwidth, % 如果在单栏模式下希望宽度为整页
]
\textbf{You are an expert in digital environment task analysis. Based on the provided information, complete two tasks:}

\textbf{Information provided:}
1)previous\_actions: A sequence of already completed actions.
2)a screenshot: The current device screen.

\textbf{Task 1: Describe the Sequence of Actions}
Describe the operation sequence as a coherent narrative.

- Format:You should return following string:
 \quad \quad description: (The current state of the system based on the screenshot)+(Describe the sequence of actions, transforming the fragmented steps into a natural language narrative) + (and is ready to proceed with [current action])

 
- Confirm the current state using the screenshot; only describe executed actions. Do not imagine or describe unexecuted steps.


- Note: If the last action in the sequence is 'Done,' add: "the system considers the task complete."

\textbf{Task 2: Understand the Sequence of Actions}
Interpret the action sequence to determine its goal.

- Format:You should return following string:\\
 objective\_thought: (Explain how you deduce the purpose of these actions, step by step.)

 
objective\_predict: (Predict the goal these actions aim to achieve.)


- Base your interpretation logically on the provided sequence. The objective\_predict must only rely on the given actions and should not include imagined or unexecuted steps.
\end{tcolorbox}
% 补充这里的内容
\subsection*{A.3\ \ \ Training Details}

For model training, we conducted full parameter fine-tuning on a robust hardware setup: six NVIDIA A100 GPUs, each equipped with 40GB of memory. An effective total batch size of 6 for Qwen3-VL-8B, OS-Atlas-Base-7B and 8 for InternVL2.5-4B was maintained throughout the process, facilitated by setting \texttt{gradient\_accumulation\_steps} to 8. The model underwent training for $2.0$ epochs, utilizing a cosine learning rate scheduler that included an initial warmup phase. To ensure efficient memory management during training, we leveraged Deepspeed with its Zero3 optimization. Our fine-tuning strategy specifically involved freezing the vision tower and multi-modal projector components, while allowing the language model to be fully fine-tuned. Training was conducted using BF16 precision and was successfully completed within 8 hours.
% 补充这里的内容
\subsection*{A.4\ \ \ Prompt Details}

We unify the agent's four capabilities (planning, grounding, description, and intent understanding) into a system prompt, and use different user prompts during training to distinguish between different task types. This approach effectively enhances all four capabilities of the agent simultaneously, leading to a more versatile and robust agent that can handle a wider range of complex tasks in diverse digital environments.

The system and user prompts used for training the Iron framework are listed below.
\begin{tcolorbox}[
    % colback=gray!5!white, % 背景颜色已移除
    colframe=black, % 边框颜色设置为黑色
    title=\textbf{\textit{System Prompt}}, % 标题
    fonttitle=\bfseries\rmfamily, % 标题字体
    arc=2mm, % 圆角
    boxsep=1mm, % 边框与内容间距
    left=3mm, right=3mm, top=2mm, bottom=2mm, % 内部填充
    breakable=true, % 允许跨页断开
    sharp corners=west, % 例如：只有左侧为直角
    % width=\columnwidth, % 如果在双栏模式下希望宽度为单栏
    % width=\textwidth, % 如果在单栏模式下希望宽度为整页
]
\textbf{You are a versatile virtual assistant for desktop, Android, and web environments, capable of task planning and intent understanding. Your four core capabilities are:}

\par % 对应原文本的 \n\n，用于在标题与列表之间创建空行

 % 使用 enumerate 环境创建编号列表 (1., 2., 3., 4.)

 \textbf{1. Task Planning.} When inputs contain ``[Task Type:Task Planning]'':
    \begin{itemize} % 使用 itemize 环境创建无序列表 (项目符号)
        \item Generate the next PyAutoGUI action based on user instruction, previous actions, and current screenshot.
        
        \item ONLY propose one action at a time.
    \end{itemize}
    Format:\\ % 格式说明部分
    \quad Thought: \textless analysis\textgreater{}\\
    \quad Action: \texttt{code\_block}

\par % 在不同的能力之间创建空行

\textbf{2. Intent Understanding.} When inputs contain ``[Task Type:Intent Understanding]'':
    \begin{itemize}
        \item Interpret the action sequence to predict its objective.
        
        \item Base prediction solely on executed actions.
    \end{itemize}
    Format:\\
    \quad objective\_thought: \textless your reasoning\textgreater{}\\
    \quad objective\_predict: \textless predicted goal\textgreater{}

\par % 在不同的能力之间创建空行

\textbf{3. Element Grounding.} When inputs contain ``[Task Type:Element Grounding]'':
    \begin{itemize}
        \item Identify the target GUI element (e.g., buttons, icons, text fields) from the instruction.
        
        \item Convert the instruction into a PyAutoGUI action.
    \end{itemize}
    Format:\\
    \textless pyautogui action code\textgreater{}

\par % 在不同的能力之间创建空行

\textbf{4. State Description.} When inputs contain ``[Task Type:State Description]'':
    \begin{itemize}
        \item Describe the current system state by observing the screenshot and action sequence.
        
        \item Highlight any potentially failed actions.
        
        \item Mark completion state by outputting "the system considers the task complete" when applicable.
        
        \item If no previous actions, output "the system has no previous actions."
        
    \end{itemize}
    Format:
    description:\\ \textless screenshot\_description\textgreater{}+\textless if completed\textgreater{}

\end{tcolorbox}

The user prompts are categorized into four types, each corresponding to a distinct task. Our Iron training framework simultaneously trains the agent's four capabilities.
\begin{tcolorbox}[
    % colback=gray!5!white, % 背景颜色已移除
    colframe=black, % 边框颜色设置为黑色
    title=\textbf{\textit{User Prompt [Planning]}}, % 标题
    fonttitle=\bfseries\rmfamily, % 标题字体
    arc=1mm, % 圆角
    boxsep=1mm, % 边框与内容间距
    left=2mm, right=2mm, top=1mm, bottom=1mm, % 内部填充
    breakable=true, % 允许跨页断开
    sharp corners=west, % 例如：只有左侧为直角
    % width=\columnwidth, % 如果在双栏模式下希望宽度为单栏
    % width=\textwidth, % 如果在单栏模式下希望宽度为整页
]
[ Task Type: Task Planning ] Please generate the next move according to the UI screenshot, instruction and previous actions. Instruction: \textless instruction\textgreater{} Given the current screen \textless screenshot\textgreater{}, previous actions: \textless previous actions\textgreater{}
\end{tcolorbox}

\begin{tcolorbox}[
    % colback=gray!5!white, % 背景颜色已移除
    colframe=black, % 边框颜色设置为黑色
    title=\textbf{\textit{User Prompt [Intent]}}, % 标题
    fonttitle=\bfseries\rmfamily, % 标题字体
    arc=1mm, % 圆角
    boxsep=1mm, % 边框与内容间距
    left=2mm, right=2mm, top=1mm, bottom=1mm, % 内部填充
    breakable=true, % 允许跨页断开
    sharp corners=west, % 例如：只有左侧为直角
    % width=\columnwidth, % 如果在双栏模式下希望宽度为单栏
    % width=\textwidth, % 如果在单栏模式下希望宽度为整页
]
[ Task Type: Intent Understanding ] Please analyze previous actions and screenshot,describe the current state,and deduce the goal of these actions by thinking step by step. Previous actions:\textless previous actions\textgreater{}
\end{tcolorbox}

\begin{tcolorbox}[
    % colback=gray!5!white, % 背景颜色已移除
    colframe=black, % 边框颜色设置为黑色
    title=\textbf{\textit{User Prompt [Grounding]}}, % 标题
    fonttitle=\bfseries\rmfamily, % 标题字体
    arc=1mm, % 圆角
    boxsep=1mm, % 边框与内容间距
    left=2mm, right=2mm, top=1mm, bottom=1mm, % 内部填充
    breakable=true, % 允许跨页断开
    sharp corners=west, % 例如：只有左侧为直角
    % width=\columnwidth, % 如果在双栏模式下希望宽度为单栏
    % width=\textwidth, % 如果在单栏模式下希望宽度为整页
]
[ Task Type: Element Grounding ] Please complete the instruction. Instrution:\textless instruction\textgreater{}
\end{tcolorbox}



\begin{tcolorbox}[
    % colback=gray!5!white, % 背景颜色已移除
    colframe=black, % 边框颜色设置为黑色
    title=\textbf{\textit{User Prompt [Desription]}}, % 标题
    fonttitle=\bfseries\rmfamily, % 标题字体
    arc=1mm, % 圆角
    boxsep=1mm, % 边框与内容间距
    left=2mm, right=2mm, top=1mm, bottom=1mm, % 内部填充
    breakable=true, % 允许跨页断开
    sharp corners=west, % 例如：只有左侧为直角
    % width=\columnwidth, % 如果在双栏模式下希望宽度为单栏
    % width=\textwidth, % 如果在单栏模式下希望宽度为整页
]
[ Task Type: State Description ] Please describe the Screenshot. Previous actions: \textless previous actions\textgreater{}
\end{tcolorbox}



\section*{B\ \ \ The MCTS Algorithm and  Hyperparameters}

\subsection*{B.1\ \ \ Algorithmic Workflow}

A detailed overview of our algorithm, which orchestrates the dual learning process to generate high-quality self-training data, is provided in the pseudocode. This algorithm is the cornerstone of our framework, enabling the agent to learn from both successful and failed experiences through our stepwise cycle-consistent reward and hindsight reproduction mechanism. For a complete understanding of its operational flow and key components, please refer to Algorithm~\ref{alg:mcts_dual_learning_optimized_detail}.
\begin{algorithm}[htbp] % 保持用户指定的浮动位置
\caption{MCTS-Guided Dual Learning (Optimized Detail)} % 调整标题
\label{alg:mcts_dual_learning_optimized_detail}
\begin{algorithmic}[1]
\STATE \textbf{Input:} Initial Policy $\pi$, Model $\mathcal{D}$, Match function, Task Dataset $\mathcal{D_T}$, Iterations $N$, Batch size $B$, MCTS Depth $T$, Replay Buffer $B_{replay}$. \textbf{Output:} Trained $\pi$ and $\mathcal{D}$. % 合并输入输出，节省一行

\FOR {$i = 1$ to $N$}
    \STATE Sample batch of $B$ tasks from $\mathcal{D_T}$.
    \FOR {each task in batch}
        \STATE Initialize root node $h_0$.
        \FOR {$t = 1$ to $T$} % MCTS 树遍历循环
            \STATE \textbf{Selection:} Traverse tree to leaf node $s_t$.
            \STATE \textbf{Expansion:} Generate actions $\{a_{t}^{j}\} = \pi(I, \tau_{t-1}, o_t)$.
            \STATE \textbf{Stepwise Cycle-Consistent Reward:} $\mathcal{Q}(s_t, a_{t}^{j}) = \text{\textit{Match}}(I, \mathcal{D}(o_t, \tau_{t-1}, a_{t}^{j}))$. % 奖励计算清晰简洁
            \STATE \textbf{Backpropagation:} Update node values using $\mathcal{Q}(s_t, a_{t}^{j})$.
        \ENDFOR
        \STATE Collect best rollout $\tau = (I, \tau_{seq}, o_{end})$ and add to $\mathcal{T}_{collected}$.
    \ENDFOR

    \STATE \textbf{Data Processing:} For each trajectory $\tau \in \mathcal{T}_{collected}$:
    \STATE \quad Perform \textbf{Hindsight Reproduction} on failed $\tau$. % 反向重现更简洁.
    \STATE \quad Filter $\tau$ using 5 invalidity metrics. Add valid $\tau$ to $B_{replay}$.
    
    \STATE \textbf{Policy Optimization:} Jointly optimize $\pi$ and $\mathcal{D}$ using data from $B_{replay}$.
\ENDFOR
\end{algorithmic}
\end{algorithm}


This algorithm outlines an MCTS-guided dual learning framework designed to iteratively train a general LLM policy ($\pi$) and an intent understanding model ($\mathcal{D}$). Each iteration begins with Monte Carlo Tree Search (MCTS) to generate task trajectories. Within MCTS, actions are expanded by $\pi$, and a cycle-consistent reward ($\mathcal{Q}$ value)—derived from the semantic match between the user instruction and $\mathcal{D}$'s understood intent—guides node value updates and backpropagation.

Collected trajectories are then undergo comprehensive data processing and augmentation. This stage includes performing Hindsight Reproduction on failed paths to transform them into usable training data, generating specific data for Instruction Grounding and Intent Understanding , and filtering by predefined metrics before storage in a replay buffer. Ultimately, the algorithm jointly optimizes policy $\pi$ (for planning and instruction grounding) and the intent understanding model $\mathcal{D}$, fostering their mutual enhancement and synergistic improvement.

\subsection*{B.2\ \ \ Selection of Node Count}

In our experimental setup, we empirically determined that generating exactly 7 child nodes per decision step achieves the optimal balance for exploration efficiency. Through systematic iterative testing, we observed that configurations with fewer than 7 nodes (e.g., 5–6) consistently yielded insufficient trajectory diversity, critically limiting the agent's ability to discover varied solution paths in complex sequential tasks such as multi-step web navigation. Conversely, exceeding 7 nodes (e.g., 8–9) introduced two fundamental challenges: (1) reduced computational efficiency due to increased redundant action sequences that wasted resource allocation, and (2) degraded data quality manifested through invalid trajectories (e.g., attempts to interact with non-existent UI elements) and hallucination phenomena, which directly compromised training reliability. Validated across diverse task environments including web operation and logical reasoning scenarios, the 7-node threshold represents a practical equilibrium that maximizes exploration breadth while maintaining execution stability—without inducing redundancy or data corruption. This parameter selection, grounded in empirical sensitivity analysis, aligns with the fundamental exploration-exploitation trade-offs inherent in sequential decision-making frameworks.

\subsection*{B.3\ \ \ Maximum Search Tree Depth}

In the OSWorld environment, we use a noun-based method to determine task difficulty, classifying tasks into three categories: easy, medium, and hard. The corresponding maximum search depths are set to 15, 30, and 45. Conversely, in the AndroidWorld environment, the maximum depth is defined based on the number of built-in task steps provided with the task.


\subsection*{B.4 \quad Analysis of MCTS Efficiency and Data Generation Cost}
\label{ssec:mcts_efficiency}

\noindent\textbf{MCTS Efficiency Analysis.}
Although \textit{Iron} employs Monte Carlo Tree Search (MCTS) for autonomous trajectory exploration, the search process is only used during the self-training data generation stage and does not introduce additional inference overhead during deployment. To better understand the computational cost of our framework, we estimate the time and resource consumption required to generate the self-training trajectories.

For a fair comparison, we evaluate the cost of obtaining 5k successful trajectories, including interaction time, environment execution, and model inference cost. The estimation follows the same evaluation environment and inference configuration used in our experiments. As shown in Table~\ref{tab:mcts_cost}, \textit{Iron} requires comparable time to existing agent-based data collection approaches while avoiding expensive human annotation or proprietary API expenses.

\begin{table}[h]
\centering
\small
\begin{tabular}{lcc}
\toprule
\textbf{Method} & 
\textbf{Time Effort (h)} &
\textbf{API Cost (\$)}
\\
\midrule
Human Annotation 
& 2000 
& 0
\\

GPT-4o Agent
& 396
& 1968
\\

Claude-Opus Agent
& 310
& 9900
\\

\textit{Iron}
& 343
& 0
\\

\bottomrule
\end{tabular}
\caption{
Estimated cost for collecting 5k successful trajectories.
\textit{Iron} avoids external API costs by using open-source foundation models while maintaining competitive trajectory generation efficiency.
}
\label{tab:mcts_cost}
\end{table}


\noindent\textbf{Discussion.}
The main computational cost of \textit{Iron} comes from the offline self-training stage, where MCTS explores multiple candidate trajectories and selects high-quality solutions through the SCC reward mechanism. However, this cost is amortized because the generated trajectories are reused for subsequent supervised optimization and do not require repeated online search.

Compared with human annotation, \textit{Iron} reduces the reliance on expensive manual demonstrations. Compared with closed-source agent generation, \textit{Iron} eliminates API expenses while achieving similar data generation efficiency. More importantly, unlike random trajectory collection, MCTS provides structured exploration and failure recovery, enabling the collected trajectories to contain diverse and informative behaviors.

Therefore, although MCTS introduces additional computation during training, it provides a scalable mechanism for autonomous data generation and is essential for enabling the self-improvement capability of \textit{Iron}.

\section*{C \quad Stepwise Cycle-Consistent Reward Details}
\subsection*{C.1\ \ \ Prompt for Calculating the Matching Score}

To ensure a robust and objective evaluation of our agent's intent understanding, we devised a specialized prompt to calculate the semantic matching score between a high-level user instruction and a sequence of executed actions. This prompt, which is designed to guide a scoring model, is presented in full below:

\begin{tcolorbox}[
    % colback=gray!5!white, % 背景颜色已移除
    colframe=black, % 边框颜色设置为黑色
    title=\textbf{\textit{System prompt [compute matching score]}}, % 标题
    fonttitle=\bfseries\rmfamily, % 标题字体
    arc=1mm, % 圆角
    boxsep=1mm, % 边框与内容间距
    left=2mm, right=2mm, top=1mm, bottom=1mm, % 内部填充
    breakable=true, % 允许跨页断开
    sharp corners=west, % 例如：只有左侧为直角
    % width=\columnwidth, % 如果在双栏模式下希望宽度为单栏
    % width=\textwidth, % 如果在单栏模式下希望宽度为整页
]
\textbf{You are an expert in key information extraction and semantic matching. Your task is to compare an origin instruction with a list of descriptions and assign scores based on their relevance.}
\par
\textbf{Input:}
\begin{itemize}
    \item origin\_instruction: A sentence describing the original task.
    \item descriptions: A list of sentences describing sequences of operations.
\end{itemize}
\par
\textbf{Output:} For each description in the list, provide:
\begin{itemize}
    \item Thought: Explain your reasoning for the score.
    \item Principles: State the rule(s) you followed to assign the score.
    \item Score: A specific float value between 0 and 1, representing the match level.
\end{itemize}
\par
\textbf{Scoring Rules:}
\begin{itemize}
    \item If the description opens the correct app or environment but does not address the task, score between 0.5 and 0.6.
    \item If the description finds the task object but does not meet any requirements, score between 0.6 and 0.7.
    \item If the description finds the task object and completes a small portion (less than 50\%) of the task, score between 0.7 and 0.8.
    \item If the description finds the task object and completes a large portion (50\%-90\%) of the task, score between 0.8 and 0.9.
    \item If the description finds the task object and completes more than 90\% of the task, score between 0.9 and 1.
    \item Special case: If there is only one description in the list, return one set of Thought, Principles, and Score for that description.
\end{itemize}
\par
\textbf{Important Notes:}
\begin{itemize}
    \item Return one set of Thought, Principles, and Score for each description in the input list.
    \item Scores must be unique and distinguishable (no duplicate scores).
    \item Do not use ranges like ``0.7/0.8''; return a specific float value.
    \item Do not use markdown formatting in your response.
\end{itemize}
\end{tcolorbox}

\subsection*{C.2\ \ \ Example of Stepwise Cycle-Consistent Reward}

The following is a detailed example that showcases the agent's intent alignment scoring mechanism. 

% It clearly illustrates the model's input and output formats, as well as how we assign matching scores to action sequences of varying quality. Given an original instruction and a list of action descriptions, the model outputs its reasoning process, the scoring principles it followed, and the final score, thereby validating the model's accurate understanding of the intent.

\begin{tcolorbox}[
    title=\textbf{\textit{Example: Intent Alignment Scoring}},
    colframe=black,       % 设置黑色边框
    fonttitle=\bfseries,   % 标题加粗
    arc=2mm,              % 边角圆弧
    boxrule=0.5pt,        % 边框粗细
    boxsep=1mm,
    left=2mm, right=2mm, top=1mm, bottom=1mm,
    breakable=true,
    sharp corners=west,
]
\noindent\textbf{Input:}
\begin{description}
    \item[origin\_instruction:] \texttt{Can you set the appearance color of my Chrome browser to black?}
    \item[descriptions:]\item \texttt{1. The user clicked the 'Menu' button, then selected 'Settings'. The system is ready to click 'Appearance'.}
        \item \texttt{2. The user clicked the 'Menu' button, then selected 'Settings'. The system is ready to click 'Privacy and Security'.}
        \item \texttt{3.The user clicked the 'Menu' button, then selected 'Settings'. The system is ready to click 'Extensions'.}
\end{description}

\noindent\textbf{Output:}

\begin{tcolorbox}[
    colframe=black,       % 内部框的边框颜色
    boxsep=1mm,
    boxrule=0.5pt,
    arc=0.5mm,
    breakable=true,
]
\textbf{Description 1:}
\begin{description}
    \item[Thought:] This description leads to the correct settings menu but does not change the color. It partially addresses the task.
    \item[Principles:] The description opens the correct app and finds the task object but does not meet the task requirements.
    \item[Score:] 0.70
\end{description}
\end{tcolorbox}

\begin{tcolorbox}[
    colframe=black,
    boxsep=1mm,
    boxrule=0.5pt,
    arc=0.5mm,
    breakable=true,
]
\textbf{Description 2:}
\begin{description}
    \item[Thought:] This description navigates to 'Privacy and Security', which is unrelated to changing the appearance color.
    \item[Principles:] The description opens the correct app but diverges from the task requirements.
    \item[Score:] 0.55
\end{description}
\end{tcolorbox}

\begin{tcolorbox}[
    colframe=black,
    boxsep=1mm,
    boxrule=0.5pt,
    arc=0.5mm,
    breakable=true,
]
\textbf{Description 3:}
\begin{description}
    \item[Thought:] This description navigates to 'Extensions', which is unrelated to changing the appearance color.
    \item[Principles:] The description opens the correct app but does not address the task requirements.
    \item[Score:] 0.58
\end{description}
\end{tcolorbox}

\end{tcolorbox}

\subsection*{C.3 \quad SCC Reward Analysis}
\label{sec:scc_reward_analysis}

\noindent\textbf{Motivation.}
The effectiveness of autonomous self-training largely depends on the quality of generated trajectories. However, task success signals in digital environments are usually sparse and only available after task completion, making it difficult to provide reliable guidance during exploration. To address this limitation, we introduce the Stepwise Cycle-Consistent (SCC) reward, which measures whether the intermediate reasoning process remains semantically aligned with the original instruction.


\noindent\textbf{Empirical Validation of SCC Reward.}
To verify that SCC provides meaningful guidance rather than serving as an arbitrary heuristic, we analyze the correlation between SCC scores and downstream task performance. Specifically, we calculate the average SCC score of generated trajectories and measure its relationship with MCTS success rate on OSWorld and AndroidWorld. As shown in Table~\ref{tab:scc_validation}, SCC scores consistently increase with more self-training iterations and exhibit a strong positive correlation with task success, demonstrating that higher semantic consistency corresponds to better trajectory quality.

\begin{table}[t]
\centering
\small
\begin{tabular}{c|c|c|c|c}
\toprule
\textbf{Iter.} &
\textbf{SCC} &
\textbf{Match Acc.} &
\textbf{OSWorld} &
\textbf{AndroidWorld}
\\
\midrule
5k  & 0.45 & 74.5\% & 0.48 & 17.50\% \\
10k & 0.58 & 81.0\% & 0.62 & 18.09\% \\
20k & 0.72 & 88.5\% & 0.74 & 19.51\% \\
30k & 0.84 & 92.5\% & 0.82 & 21.13\% \\
\bottomrule
\end{tabular}
\caption{
Validation of SCC reward. Higher SCC scores consistently correspond to improved intent matching accuracy and task success rates, indicating that SCC is a reliable indicator of trajectory quality.
}
\label{tab:scc_validation}
\end{table}

\noindent\textbf{Why SCC Reward Helps.}
Different from sparse terminal rewards, SCC provides dense intermediate supervision during exploration. It encourages the agent to preserve the correspondence between high-level instructions and low-level actions, reducing semantic drift and ineffective exploration. Moreover, SCC does not require human preference labels or external reward models, enabling fully autonomous trajectory generation.

\noindent\textbf{Relationship with Self-training.}
In our framework, SCC reward is mainly used for MCTS trajectory evaluation and selection. High-quality trajectories with strong semantic consistency are retained as self-training samples, while low-quality trajectories are filtered or regenerated. Therefore, SCC serves as an internal quality estimator that enables reliable autonomous data generation rather than an additional supervised signal requiring external resources.

\section*{D \quad Supplementary Procedures for Hindsight Reproduction and Trajectory Filtering}
\subsection*{D.1\ \ \ Self-Prompting Mechanism}

To effectively train our agent's intent understanding capability without relying on costly human annotations, we devised a novel method for generating ground truth data. This approach leverages a self-prompting mechanism where the agent itself provides the necessary annotations. Specifically, we employ a self-reflective prompting at state \(s_{t+1}^i\), which results from executing the action \(a_t^i\), to provide reference for understanding the low-level sequences $\tau_{{t}}^{i}=\{a_0, a_1, \ldots, a_{t-1}\ ,a_{t}^{i}\}$.  we prompt the agent with the following instruction:\texttt{“ Please describe the current state
and the goals achieved according to the
screenshot.”} The response serves as the ground truth for the intent understanding of the action sequence up to time \(t\).

\subsection*{D.2\ \ \ Trajectory Filtering Metrics}
To address the complexity of digital environments, we introduce five metrics to filter out problematic trajectories caused by unpredictable feedback loops (e.g., repeated actions) or external factors (e.g., network issues):

\begin{itemize}
\item[-] \textit{Repeatability}: proportion of highly repetitive actions. We calculate the proportion of actions that are both semantically and behaviorally similar based on the intent description $U_{end}$ and action sequence $\tau_{end}$ of the entire trajectory, with values ranging from 0 to 1, where higher scores indicate excessive repetition.
\item[-] \textit{Ineffectiveness}: proportion of ineffective actions. We categorize actions such as \texttt{go back}, \texttt{go forward}, and \texttt{page close} as ineffective in the action sequence to prevent redundancy and misleading signals caused by excessive occurrences of these actions. This metric is normalized between 0 and 1, with higher values signaling more invalid actions.
\item[-] \textit{Exploratory}: proportion of exploratory actions. We label actions such as \texttt{scroll}, \texttt{new tab}, and \texttt{hover} as exploratory in the action sequence. Excessive occurrences of these actions can also lead to redundancy and misleading signals. This metric is normalized between 0 and 1, with higher values signaling more exploratory actions.
\item[-] \textit{Logicality}: logical Consistency of action sequences. We assess whether the execution logic aligns with human cognitive patterns by analyzing the trajectory's intent description $U_{end}$ and action sequence $\tau_{end}$. This metric is normalized between 0 and 1 to quantify deviations from intuitive human behavior. A higher score indicates greater alignment with human logic.
\item[-] \textit{Invalidity}: invalidity of the final outcome. This metric evaluates whether the final observation $o_{end}$ after execution invalidates. If the observation indicates issues such as network connection errors or 404 errors, which lack meaningful reference value, it is flagged as invalid. The metric returns a boolean value (True or False).

\end{itemize}



\begin{figure}[t]
  \centering
  \includegraphics[width=0.98\linewidth]{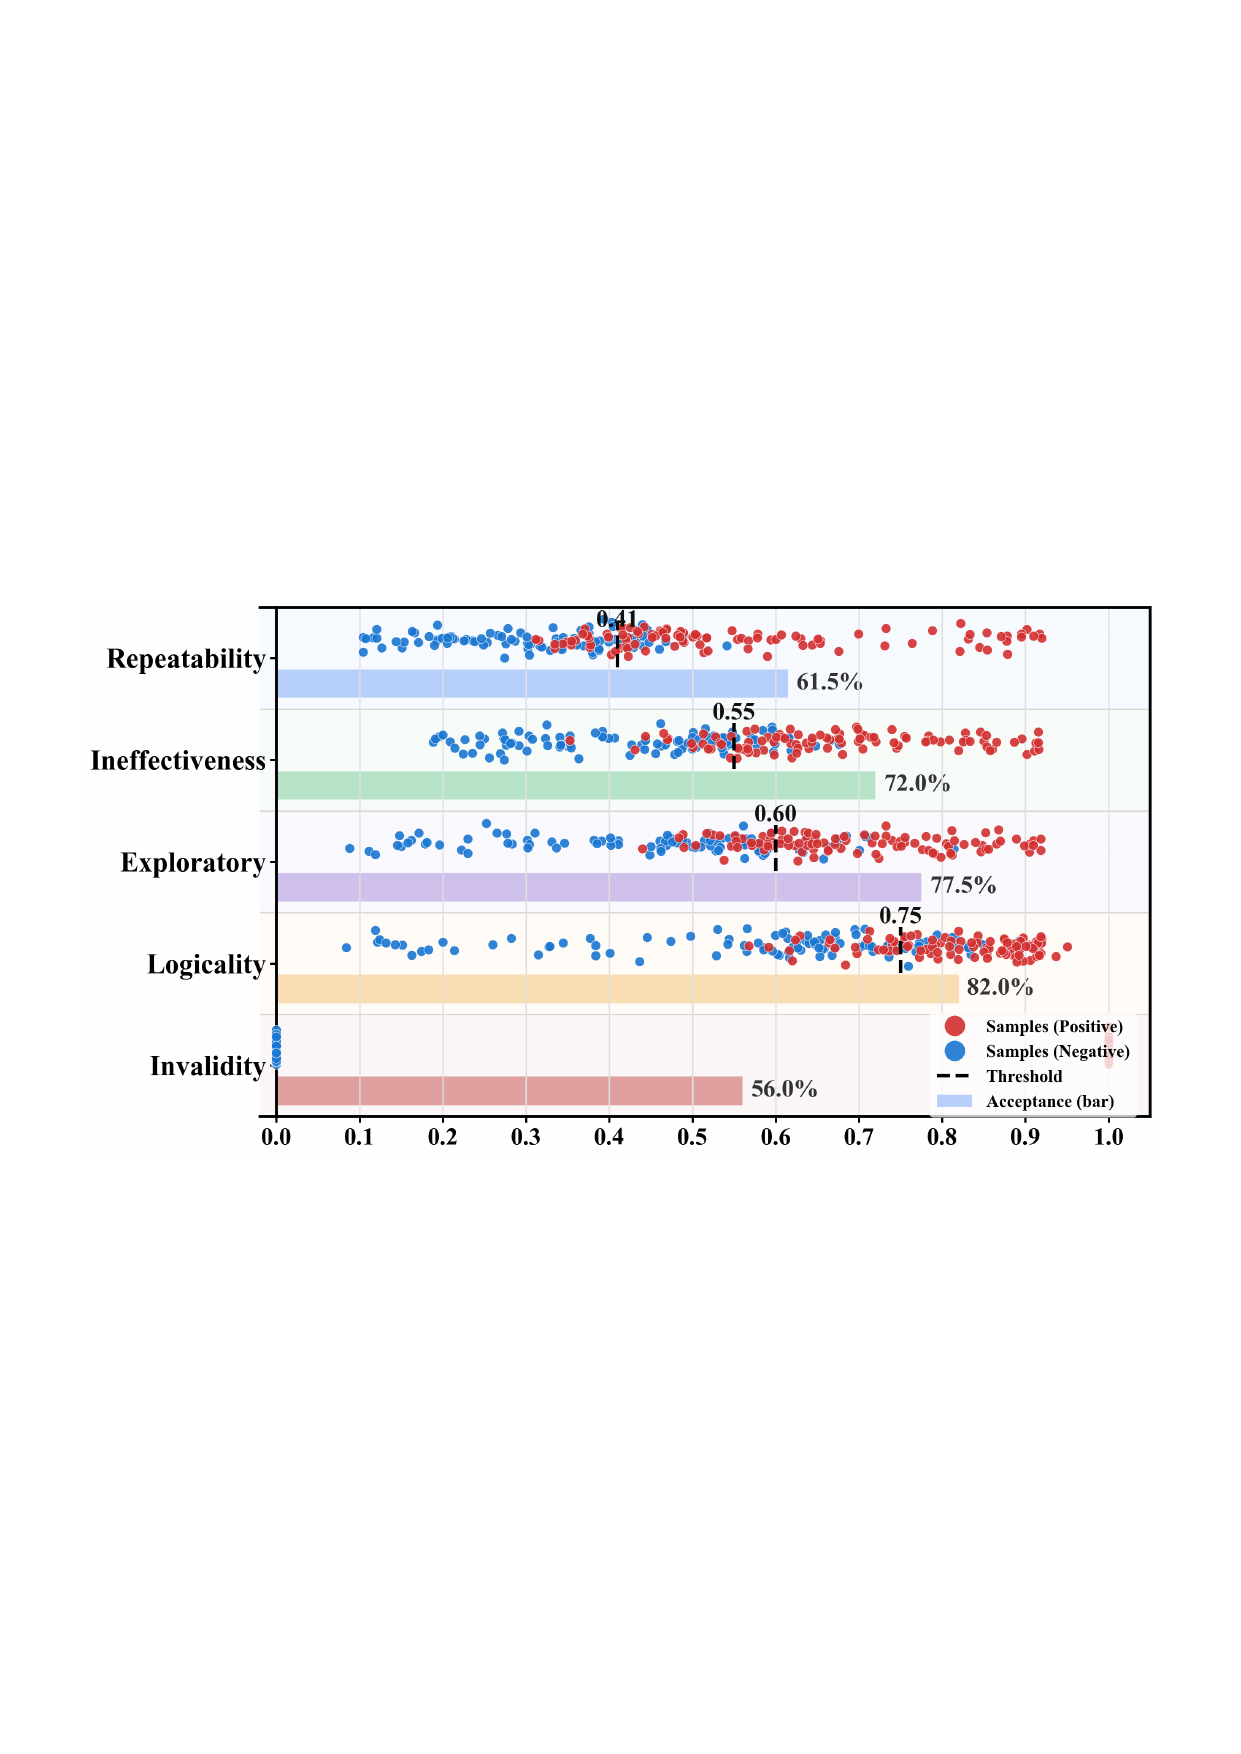}
  \caption{Visualization of five trajectory filtering metrics. The bar chart shows the human-evaluated acceptability rates after ablating each single metric (56.0\%–82.0\%). The scatter plot confirms all thresholds are experimentally optimized.}
  \label{fig:indicator_scatter}
\end{figure}

\subsection*{D.3 \quad Filtering Calculate Method}
To mitigate the distribution shifts induced by hindsight relabeling and construct a high-quality self-training dataset, we propose a \textbf{rigorous five-metric joint filtering pipeline} with all thresholds \textbf{optimized via quantitative experiments} (instead of manual arbitrary settings). A trajectory is only admitted for training if it satisfies \textbf{all five criteria simultaneously}; violating any single metric results in direct rejection of the entire trajectory.

As visualized in Figure \ref{fig:indicator_scatter}, we conduct ablation experiments and human evaluations on 200 sampled trajectories to validate the filtering metrics. The figure integrates two core analyses: (1) the horizontal bar chart quantifies the trajectory acceptability rate after removing each individual filtering metric (ranging from 56.0\% to 82.0\%), demonstrating an obvious performance drop without any metric; (2) the scatter plot verifies that all metric thresholds are experimentally optimized to optimal values rather than manual configuration.

The concrete filtering rules with \textbf{experimentally determined thresholds} are defined as follows:
\begin{itemize}
    \item \textbf{Repeatability}: Score $\leq \boldsymbol{0.41}$, filtering out trajectories with repetitive and meaningless actions;
    \item \textbf{Ineffectiveness}: Score $\leq \boldsymbol{0.55}$, eliminating trajectories with invalid and low-efficiency behaviors;
    \item \textbf{Exploratory}: Score $\leq \boldsymbol{0.60}$, retaining purposeful exploration instead of aimless wandering;
    \item \textbf{Logicality}: Score $\geq \boldsymbol{0.75}$, ensuring action sequences align with human cognitive logic;
    \item \textbf{Invalidity}: Trajectory must pass the binary validity check (classified as valid).
\end{itemize}

This strict filtering mechanism excludes flawed and misleading data caused by distribution shifts, which is critical for enhancing the robustness and reliability of our self-training framework.
% 补充这里的内容


\subsection*{D.4 \quad Semantic Accuracy Analysis of Hindsight Reproduction}
\label{sec:hindsight_accuracy}

\noindent\textbf{Motivation.}
Hindsight reproduction is introduced to recover failed trajectories by reconstructing the underlying intent and generating alternative action sequences. However, directly relying on the predicted intent may introduce semantic hallucinations or overly abstract descriptions. Therefore, we further analyze the semantic reliability of reproduced trajectories.

\begin{figure}[t]
    \centering
    \includegraphics[width=0.5\linewidth]{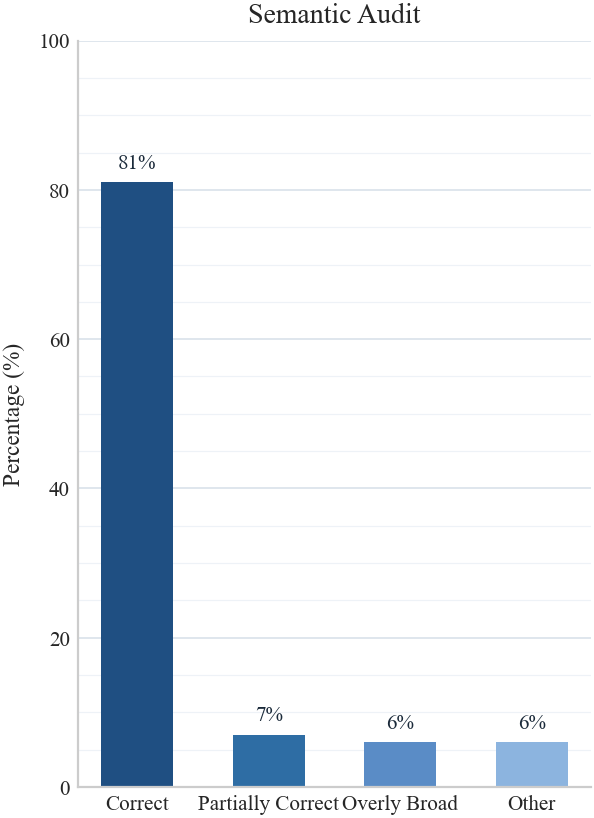}
    \caption{
    Human evaluation of 100 hindsight-reproduced trajectories.
    Most reproduced intents preserve the original task semantics, with only a small portion exhibiting overly broad or incomplete descriptions.
    }
    \label{fig:semantic_audit}
\end{figure}


\noindent\textbf{Objective Grounding.}
To reduce the risk of intent hallucination, the reproduced training samples are not generated from intent representations alone. Specifically, each reproduced trajectory jointly considers:
(1) the original task instruction,
(2) the inferred intent representation, and
(3) the corresponding low-level action sequence and screen observations.

By grounding the inferred intent with observable interaction traces, the generated trajectories preserve the connection between high-level objectives and executable behaviors, preventing the model from learning unsupported semantic abstractions.

\noindent\textbf{Human Semantic Audit.}
To quantitatively evaluate the semantic consistency of hindsight reproduction, we randomly sampled 100 reproduced trajectories and conducted human evaluation. Each trajectory was compared with the original task instruction and inferred intent, and annotated according to whether the reproduced intent accurately reflected the original objective.

As shown in Fig.~\ref{fig:semantic_audit}, 88\% of reproduced trajectories maintain consistent semantic meanings with the original intent, while only 6\% contain overly broad descriptions. The remaining cases mainly involve partially incomplete but still task-related intent descriptions. These results demonstrate that hindsight reproduction introduces limited semantic drift and provides reliable supervision for self-training.



\noindent\textbf{SCC-based Safeguard.}
Besides explicit semantic auditing, our SCC reward provides an additional automatic safeguard during self-training. Since SCC measures the consistency between the original instruction and inferred intent, trajectories containing inconsistent or hallucinated intents naturally receive lower SCC scores. Such trajectories are therefore less likely to be selected by MCTS evaluation and trajectory filtering, reducing the propagation of semantic errors during iterative self-training.

\noindent\textbf{Summary.}
Overall, hindsight reproduction combines objective grounding, semantic auditing, and SCC-based filtering to ensure that generated trajectories remain aligned with the original task objective. This design enables effective failure recovery while substantially reducing semantic drift.



\section*{E \quad Details of Self-training }
\subsection*{E.1\ \ \ Training Details}
% 补充这里的内容
The training configuration was kept consistent with the imitation learning phase, with an effective batch size set to 6 for Qwen3-VL-8B, OS-Atlas-Base-7B and 8 for InternVL2.5-4B, achieved by accumulating gradients over 8 steps. All models trained using the LlamaFactory framework. The models underwent 2.0 epochs of training, employing a cosine learning rate scheduler with an initial warmup phase. For memory efficiency, we utilized \texttt{Deepspeed} with its \texttt{Zero3} optimization. Our fine-tuning strategy involved exclusively updating the language model while keeping the vision tower and multi-modal projector frozen. The training was conducted in BF16 precision and finished in under 3 hours.



% 补充这里的内容

\subsection*{E.2 \quad Impact of Iterative Training}
\par % This is for a line break before the paragraph
To validate the impact of our iterative versus non-iterative self-training methodologies on model performance, we conducted a comparative experiment on a subset of various benchmarks. The OS-Atlas-7B-\textit{Iron}-20k model was trained iteratively, while the OS-Atlas-7B-20k model was trained in a non-iterative, one-shot manner using a single batch of data. The 30k model also follows this training approach. As shown in Table~\ref{tab:iterative_vs_non_iterative}, our experimental results demonstrate that the iterative self-training approach achieved superior performance across all three environments, which strongly proves that the improvement in data quality during the self-training process is crucial for model effectiveness.






\section*{ F.1 \quad Evaluation Details}
\label{sec:evaluation_details}

This section provides detailed information on the benchmarks and baseline models used to evaluate our generalist virtual agent.

\subsection*{F.1 \quad Benchmarks}
\label{ssec:benchmarks}

We evaluate our generalist virtual agent on three diverse, cross-platform, and cross-operating system benchmarks. For primary performance assessment, we use \textbf{OSWorld} and \textbf{AndroidWorld}, while \textbf{VisualWebArena} is used to specifically test generalization to unseen environments. For all evaluations, we used a specific subset of each benchmark for testing. Our agent's interaction with these environments is based exclusively on \textbf{raw screenshots}, simulating a real-world, human-like perception modality.

\begin{itemize}
    \item \textbf{OSWorld}: OSWorld provides a rich, comprehensive environment for evaluating agents on a variety of desktop and web tasks. It serves as a crucial benchmark for assessing the agent's ability to navigate and interact with a desktop operating system interface and common applications. This benchmark is particularly valuable for testing the agent's planning and execution skills in a multi-application context.

    \item \textbf{AndroidWorld}: This benchmark is specifically designed for evaluating mobile planning tasks within the Android ecosystem. It tests the agent's proficiency in interacting with a mobile OS, including app navigation, settings adjustments, and complex multi-step tasks. AndroidWorld is essential for validating the agent's performance in mobile-first scenarios, ensuring its generalist nature extends to a different platform.

    \item \textbf{VisualWebArena}: To rigorously assess the agent's generalization capabilities to entirely novel environments, we use VisualWebArena. This is a highly challenging benchmark consisting of complex, real-world web tasks that are completely new to the agent during training. The performance on VisualWebArena is a key indicator of the agent's ability to reason and adapt to unfamiliar web layouts and task requirements without prior fine-tuning on the specific domain.
\end{itemize}


\begin{table*}[htbp]
\centering
\small
\renewcommand{\arraystretch}{1.05}
\begin{tabular}{lccc}
\toprule
Model & Success (\%) & Success Count & 95\% CI \\
\midrule

Qwen3-VL-8B-IL
&38.39
&129/336
&[33.4,43.7]
\\

Qwen3-VL-8B-\textit{Iron-10k}
&39.28
&132/336
&[34.2,44.6]
\\

Qwen3-VL-8B-\textit{Iron-20k}
&40.47
&136/336
&[35.3,45.8]
\\

Qwen3-VL-8B-\textit{Iron-30k}
&41.96
&141/336
&[36.8,47.3]
\\

Qwen3-VL-8B-\textit{Full}
&41.67
&140/336
&[36.5,47.0]
\\

Qwen3-VL-8B-\textit{DPO}
&40.18
&135/336
&[35.0,45.5]
\\

\midrule

OS-Atlas-7B-IL
&2.97
&10/336
&[1.6,5.4]
\\

OS-Atlas-7B-\textit{Iron-30k}
&5.95
&20/336
&[3.9,8.9]
\\

\midrule

InternVL2.5-4B-IL
&1.49
&5/336
&[0.6,3.5]
\\

InternVL2.5-4B-\textit{Iron-30k}
&3.87
&13/336
&[2.3,6.6]
\\

\bottomrule
\end{tabular}

\caption{
Confidence interval analysis on OSWorld.
The success count is calculated over 336 evaluation tasks.
Intervals are computed using the Wilson score interval with 95\% confidence.
}
\label{tab:confidence_interval}
\end{table*}


\subsection*{F.2 \quad Baselines}
\label{ssec:baselines_methodology}

\noindent\textbf{Baseline Selection.}
Different from task-specific methods that aim to achieve the best performance
with a particular backbone, \textit{Iron} is designed as a
\textbf{model-agnostic self-training framework} that can be integrated with
various foundation models. Therefore, our experiments are designed to verify
whether \textit{Iron} can consistently improve different base agents through
autonomous data generation and iterative self-training, rather than competing
with a specific model architecture. 

We evaluate \textit{Iron} on multiple representative vision-language agents,
including Qwen3-VL-8B, OS-Atlas-7B, and InternVL2.5-4B, covering different
model scales and architectures. For fair comparison, models within each
backbone group share the same initialization, training data scale, and
evaluation protocols. The consistent improvements across different backbone
families demonstrate the general applicability, scalability, and robustness of
\textit{Iron}.

\noindent\textbf{Baselines.}
We establish a comprehensive baseline system under unified evaluation settings,
including \textbf{closed-source foundation models}, \textbf{open-source
mainstream models}, and \textbf{controlled variants based on the same backbone}.
All models are evaluated on OSWorld (including OS, Office, Daily, Professional,
and Workflow categories) and AndroidWorld. For open-source comparisons, the
best-performing open-weight models are highlighted in bold in Table
\ref{tab:model_performance_custom}.


\begin{itemize}

    \item \textbf{Closed-source Foundation Models.}
    We include representative commercial vision-language foundation models as
    strong reference systems, including GPT-4o, GPT-4V, Gemini-ProV,
    Gemini-Pro-1.5, Claude-3-Opus, Claude-3-7-Sonnet, Claude-4-Sonnet, and
    Claude-Sonnet-4-5. These models are evaluated under the same benchmark
    protocols. Since their architectures, training data, and optimization
    procedures are inaccessible, they are used only as external performance
    references and are excluded from open-source comparisons.

    \item \textbf{Open-source Mainstream Models.}
    We evaluate representative open-source vision-language agents, including
    Qwen2.5-VL-72B, Qwen2.5-VL-32B, Qwen3-VL-8B, OS-Atlas-7B, and
    InternVL2.5-4B. These models cover different parameter scales and provide
    strong baselines for assessing the effectiveness of our self-training
    framework.

    \item \textbf{Controlled Baselines and Variants.}
    To isolate the contribution of self-training, we construct controlled
    experiments based on three backbone models: Qwen3-VL-8B, OS-Atlas-7B, and
    InternVL2.5-4B.

    \begin{itemize}

        \item \textbf{Imitation Learning (IL).}
        The IL model is trained only with the supervised imitation learning
        stage, using the same initialization and training data as its
        corresponding \textit{Iron} variant. Specifically, the IL training
        contains 210k samples, including 120k grounding samples and 90k
        planning samples from the Aguvis dataset. These models provide the
        starting point for subsequent self-training.

        \item \textbf{\textit{Iron} Variants.}
        Starting from the IL model, we progressively apply our self-training
        framework with increasing amounts of automatically generated data.
        Specifically, \textit{Iron-10k}, \textit{Iron-20k}, and
        \textit{Iron-30k} denote models trained with 10k, 20k, and 30k
        self-training trajectories, respectively. Each stage uses the previous
        checkpoint as initialization, enabling iterative improvement through
        autonomous trajectory generation, filtering, and refinement.
        \item \textbf{\textit{Full} Version.}
        We introduce a strong supervised learning baseline trained with
        3$\times$ the IL data scale (630k samples). Unlike \textit{Iron}, which
        leverages self-generated trajectories from autonomous exploration, the
        \textit{Full} version uses only additional supervised data from the original
        training source. This baseline is designed to examine whether the gains of
        \textit{Iron} come merely from increasing data volume or from the quality
        of autonomously generated training trajectories.
    
        \item \textbf{\textit{DPO} Version.}
        We include a preference optimization baseline based on Step-DPO,
        initialized from the corresponding IL model. The preference pairs are
        naturally obtained from our trajectory generation process, where
        SCC-guided selection provides relatively better and worse trajectories.
        This baseline evaluates whether direct preference optimization can achieve
        comparable improvements to our iterative self-training strategy without
        explicit trajectory generation and refinement.

    \end{itemize}
\end{itemize}
% \noindent\textbf{Our proposed method.}
%     Following the Imitation Learning stage, we introduce \textbf{\textit{Iron}}, a novel self-training framework that allows agents to learn autonomously from both successes and failures via intention-action alignment and hindsight reproduction. As a model-agnostic framework, \textbf{\textit{Iron}} provides scalable self-improvement by generating high-quality training data and learning from failures to expand agent capabilities on complex, long-horizon tasks.
%     \begin{itemize}

%     \end{itemize}

\subsection*{F.3 \quad Statistical Significance Analysis}

\label{app:statistical_analysis}

Since OSWorld is evaluated on a fixed benchmark set with deterministic task outcomes, task-level confidence intervals are more appropriate than random-seed variance. To assess the statistical reliability of our reported improvements, we further
conduct a confidence interval analysis based on the task-level success outcomes
in OSWorld. Since OSWorld consists of a fixed set of independent tasks, each
task can be regarded as a Bernoulli trial, where success and failure correspond
to binary outcomes. Given an evaluation success rate $p$ over $N$ tasks, we
compute the 95\% confidence interval using the Wilson score interval:

\begin{equation}
CI_{95\%}
=
\frac{
\hat{p}+\frac{z^2}{2N}
\pm
z\sqrt{
\frac{\hat{p}(1-\hat{p})}{N}
+
\frac{z^2}{4N^2}
}
}{
1+\frac{z^2}{N}
},
\end{equation}

where $\hat{p}$ denotes the observed success rate, $N$ is the number of
evaluation tasks, and $z=1.96$ corresponds to a 95\% confidence level.

The detailed task numbers of OSWorld are:
OS (24), Office (95), Daily (70), Professional (46), and Workflow (101),
resulting in 336 tasks in total. We report confidence intervals for the main
open-source baselines and our proposed \textit{Iron} variants below.



The confidence intervals show that the improvements introduced by
\textit{Iron} are consistent with the observed task-level outcomes.
For Qwen3-VL-8B, the proposed \textit{Iron-30k} achieves a clear improvement
over the imitation learning baseline, increasing the success rate from
38.39\% to 41.96\%. Similar trends are observed for OS-Atlas-7B and
InternVL2.5-4B, demonstrating that the improvement is not limited to a specific
backbone.

Although the confidence intervals of some neighboring variants partially
overlap due to the finite benchmark size, this is expected because OSWorld
contains only 336 tasks. Importantly, the consistent monotonic improvement
from \textit{Iron-10k} to \textit{Iron-30k} indicates that additional
self-training trajectories provide useful supervision rather than random
variation.



\subsection*{F.4 \quad A Successful Task Completion Example} 

Table \ref{tab:successful_example} presents a complete example of task execution by an iteratively trained agent, demonstrating its ability to perform a multi-step mobile interaction task—creating a new contact named "Hugo Pereira". Starting from the home screen, the agent correctly identifies and opens the Contacts app, navigates the interface to initiate contact creation, fills in the required fields (including phone number, first name, and last name), and finally saves the entry. Each step includes a screenshot of the current interface state, along with the agent’s internal thought and the corresponding action command. The successful completion of the task highlights the agent’s robust understanding of visual interfaces, effective sequential decision-making, and precise action localization, all learned through iterative training. This example reflects the agent’s capability to generalize learned behaviors to accomplish complex, real-world mobile tasks in a structured and reliable manner.



\newpage

% \begin{tabel*}
% % 定义左对齐、自动换行、顶端对齐的列

% % 定义左对齐、自动换行、顶端对齐的列
% \newcolumntype{L}[1]{>{\raggedright\arraybackslash}p{#1}}

% \begin{longtable}{L{0.1\textwidth} L{0.38\textwidth} || L{0.1\textwidth} L{0.38\textwidth}}
% \caption{\mbox{A complete task completion example from an iteratively trained model.}}
%     \label{fig:successful_example}
%     \\
%     % --- Top: 加粗外边框 ---
%     \hhline{====}
%     \endfirsthead

%     % 跨页时继续显示外框
%     % \multicolumn{4}{@{}l}{\small\textit{Continued from previous page}} \\[5pt]
%     % \hhline{:=:=::=:==:}
%     % \endhead

%     % \multicolumn{4}{r}{\small\textit{Continued on next page}} \\
%     % \hhline{:=:=::=:==:}
%     % \endfoot

%     % % --- Bottom: 加粗外边框 ---
%     % \hhline{:=:=::=:==:}
%     % \endlastfoot

%     % ============ 数据行开始 ============

%     % Row 1: Step 1 & 2
%     \raisebox{-0.5\height}{\includegraphics[width=\linewidth]{ss2.png}} &
%     \parbox[t]{\linewidth}{
%     \vspace{-3.5em}
%     \textbf{\textit{[Step1]}}\\
%         \textbf{Thought:} To create a new contact for Hugo Pereira, I need to open the Contacts app. The Contacts icon is visible on the screen, so my next logical step is to click on it. \\
%         \textbf{Action:} \texttt{pyautogui.click\\
%         (x=0.376, y=0.582)}
%     } &
%     \raisebox{-0.5\height}{\includegraphics[width=\linewidth]{ss3.png}} &
%     \parbox[t]{\linewidth}{
%     \vspace{-3.5em}
%     \textbf{\textit{[Step2]}}\\
%         \textbf{Thought:} The app is loading; need to wait for initialization to access contact creation options. \\
%         \textbf{Action:} \texttt{WAIT}
%     } \\
%     \hhline{-|-||-|-}  % 中间细线，只画在单元格之间

%     % Row 2: Step 3 & 4
%     \raisebox{-0.5\height}{\includegraphics[width=\linewidth]{ss4.png}} &
%     \parbox[t]{\linewidth}{
%         \vspace{-3.5em}
%         \textbf{\textit{[Step3]}}\\
%         \textbf{Thought:} To create a new contact, I need to click the plus button to add new entries. \\
%         \textbf{Action:} \texttt{pyautogui.click\\
%         (x=0.871, y=0.827)}
%     } &
%     \raisebox{-0.5\height}{\includegraphics[width=\linewidth]{ss5.png}} &
%     \parbox[t]{\linewidth}{
%             \vspace{-3.5em}
%         \textbf{\textit{[Step4]}}\\
%         \textbf{Thought:} Activate phone number field to proceed with contact creation. \\
%         \textbf{Action:} \texttt{pyautogui.click\\
%         (x=0.332, y=0.706)}
%     } \\
%     \hhline{-|-||-|-}

%     % Row 3: Step 5 & 6
%     \raisebox{-0.5\height}{\includegraphics[width=\linewidth]{ss6.png}} &
%     \parbox[t]{\linewidth}{
%         \vspace{-3.5em}
%         \textbf{\textit{[Step5]}}\\
%         \textbf{Thought:} Entering phone number to create \\
%         contact. \\
%         \textbf{Action:} \texttt{pyautogui.write\\
%         (message='+13920741751')}
%     } &
%     \raisebox{-0.5\height}{\includegraphics[width=\linewidth]{ss7.png}} &
%     \parbox[t]{\linewidth}{
%             \vspace{-3.5em}
%         \textbf{\textit{[Step6]}}\\
%         \textbf{Thought:} Completing contact info by filling 'First name' field. \\
%         \textbf{Action:} \texttt{pyautogui.click\\
%         (x=0.381, y=0.288)}
%     } \\
%     \hhline{-|-||-|-}

%     % Row 4: Step 7 & 8
%     \raisebox{-0.5\height}{\includegraphics[width=\linewidth]{ss8.png}} &
%     \parbox[t]{\linewidth}{
%             \vspace{-3.5em}
%         \textbf{\textit{[Step7]}}\\
%         \textbf{Thought:} Filling in 'First name' field with 'Hugo' for contact creation. \\
%         \textbf{Action:} \texttt{pyautogui.write\\
%         (message='Hugo')}
%     } &
%     \raisebox{-0.5\height}{\includegraphics[width=\linewidth]{ss9.png}} &
%     \parbox[t]{\linewidth}{
%             \vspace{-3.5em}
%         \textbf{\textit{[Step8]}}\\
%         \textbf{Thought:} Entering last name 'Pereira' to complete contact details. \\
%         \textbf{Action:} \texttt{pyautogui.write\\
%         (message='Pereira')}
%     } \\
%     \hhline{-|-||-|-}

%     % Row 5: Step 9 & 10
%     \raisebox{-0.5\height}{\includegraphics[width=\linewidth]{ss10.png}} &
%     \parbox[t]{\linewidth}{
%             \vspace{-3.5em}
%         \textbf{\textit{[Step9]}}\\
%         \textbf{Thought:} Contact details are complete; ready to save. \\
%         \textbf{Action:} \texttt{pyautogui.click\\
%         (x=0.775, y=0.098)}
%     } &
%     \raisebox{-0.5\height}{\includegraphics[width=\linewidth]{ss11.png}} &
%     \parbox[t]{\linewidth}{
%             \vspace{-3.5em}
%         \textbf{\textit{[Step10]}}\\
%         \textbf{Thought:} Contact successfully created for Hugo Pereira. \\
%         \textbf{Action:} \texttt{mobile.terminate\\
%         (status='success')}
%     } \\
%     % --- Bottom: 加粗外边框 ---
%     \hhline{====}
% \end{longtable}
% \end{tabel*}



% 定义左对齐、自动换行、顶端对齐的列
\newcolumntype{L}[1]{>{\raggedright\arraybackslash}p{#1}}

\begin{table*}[t]
    \centering
    \caption{A complete task completion example from an iteratively trained model.}
    \label{tab:successful_example}
    \begin{tabular}{L{0.1\textwidth} L{0.35\textwidth} || L{0.1\textwidth} L{0.35\textwidth}}
        % --- Top: 细横线 ---
        \hhline{====}
        
        % ============ 数据行开始 ============
        
        % Row 1: Step 1 & 2
        \raisebox{-0.5\height}{\includegraphics[width=\linewidth]{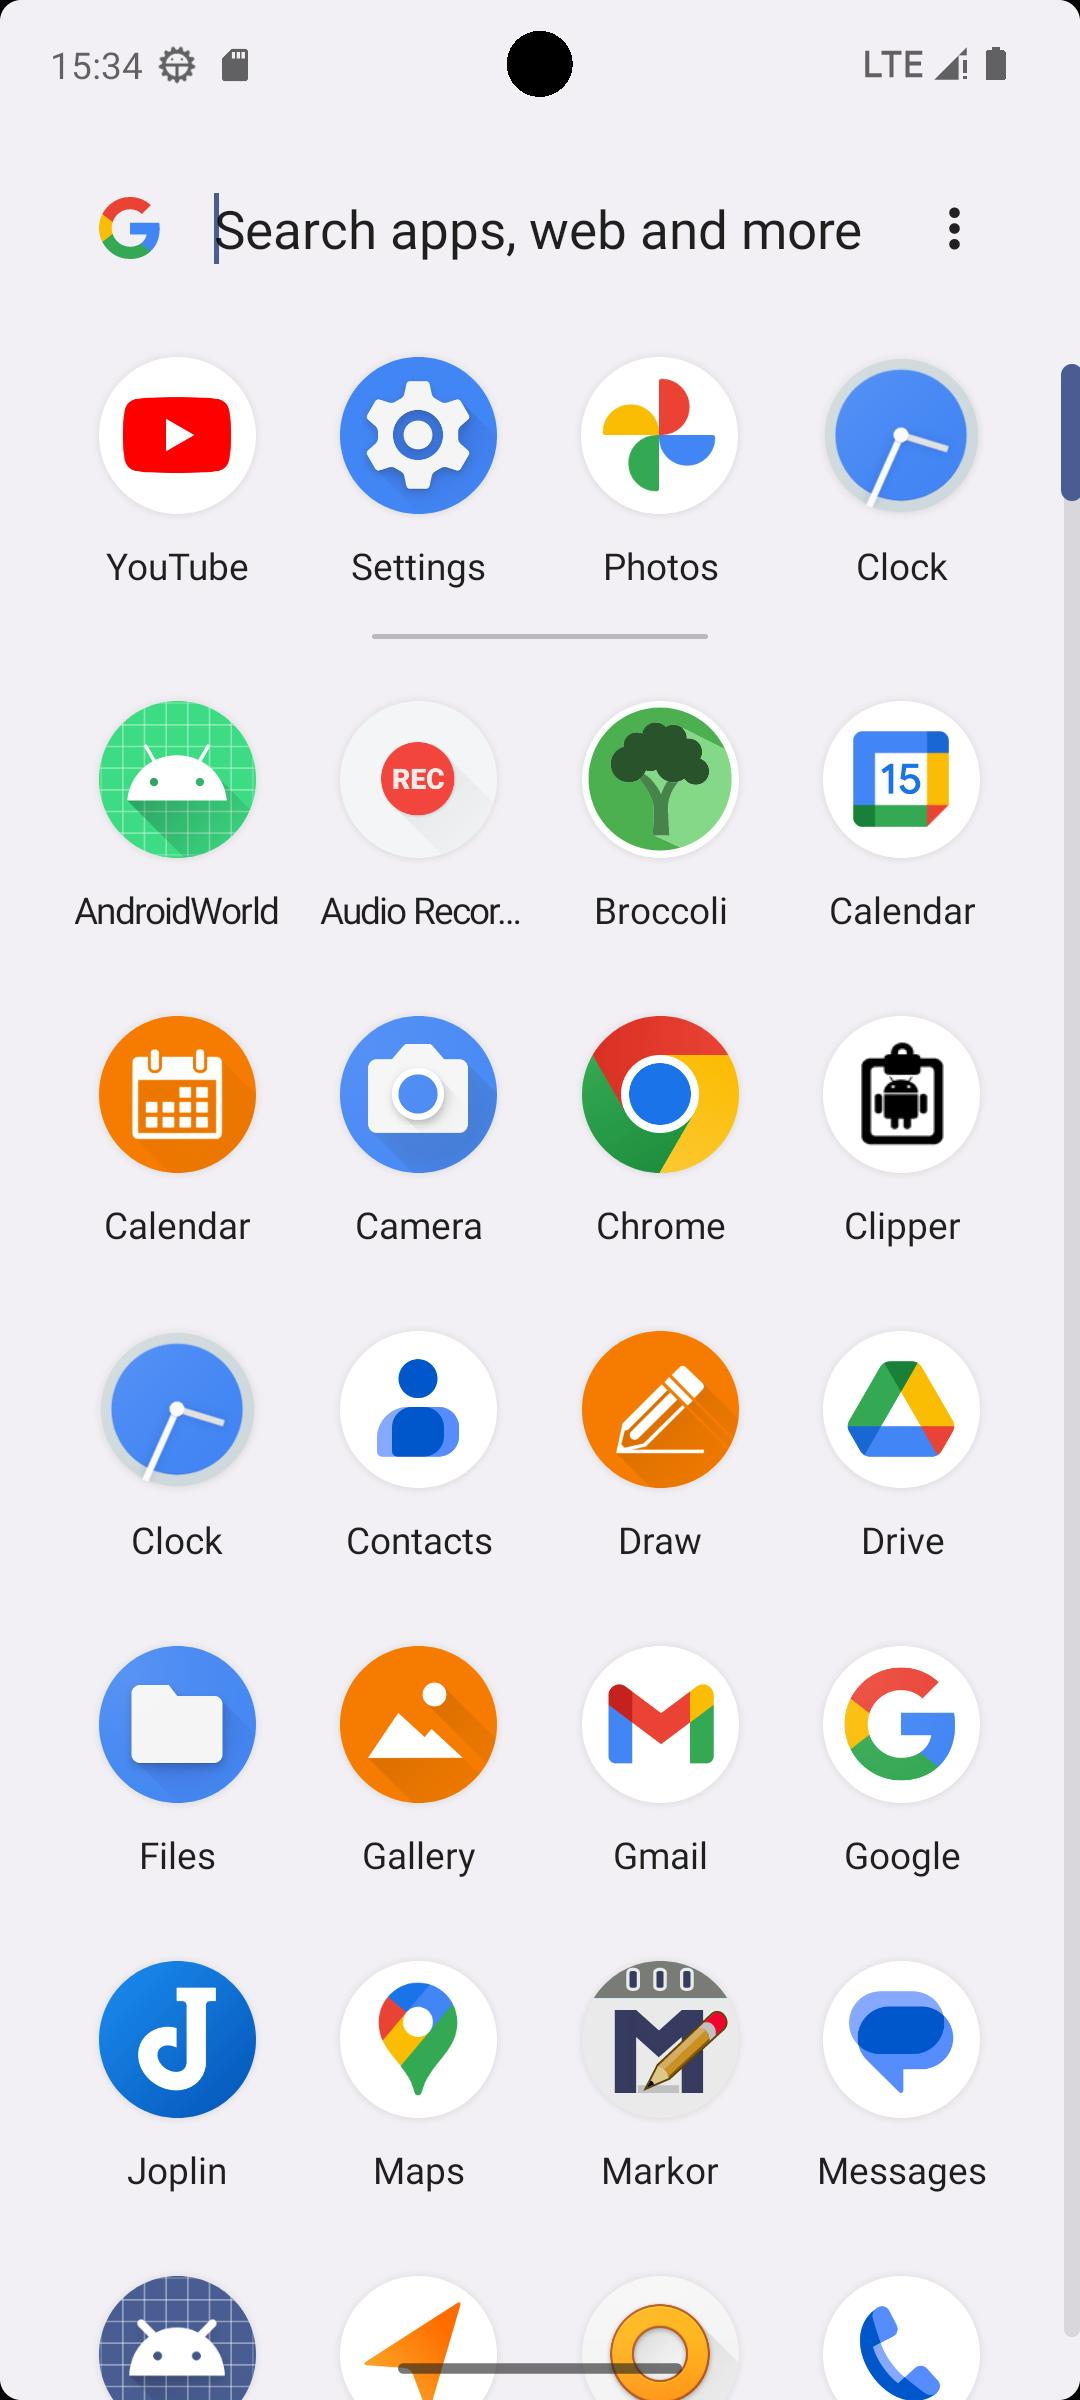}} &
        \parbox[t]{\linewidth}{
            \vspace{-3.5em}
            \textbf{\textit{[Step1]}}\\
            \textbf{Thought:} To create a new contact for Hugo Pereira, I need to open the Contacts app. The Contacts icon is visible on the screen, so my next logical step is to click on it. \\
            \textbf{Action:} \texttt{pyautogui.click\\
            (x=0.376, y=0.582)}
        } &
        \raisebox{-0.5\height}{\includegraphics[width=\linewidth]{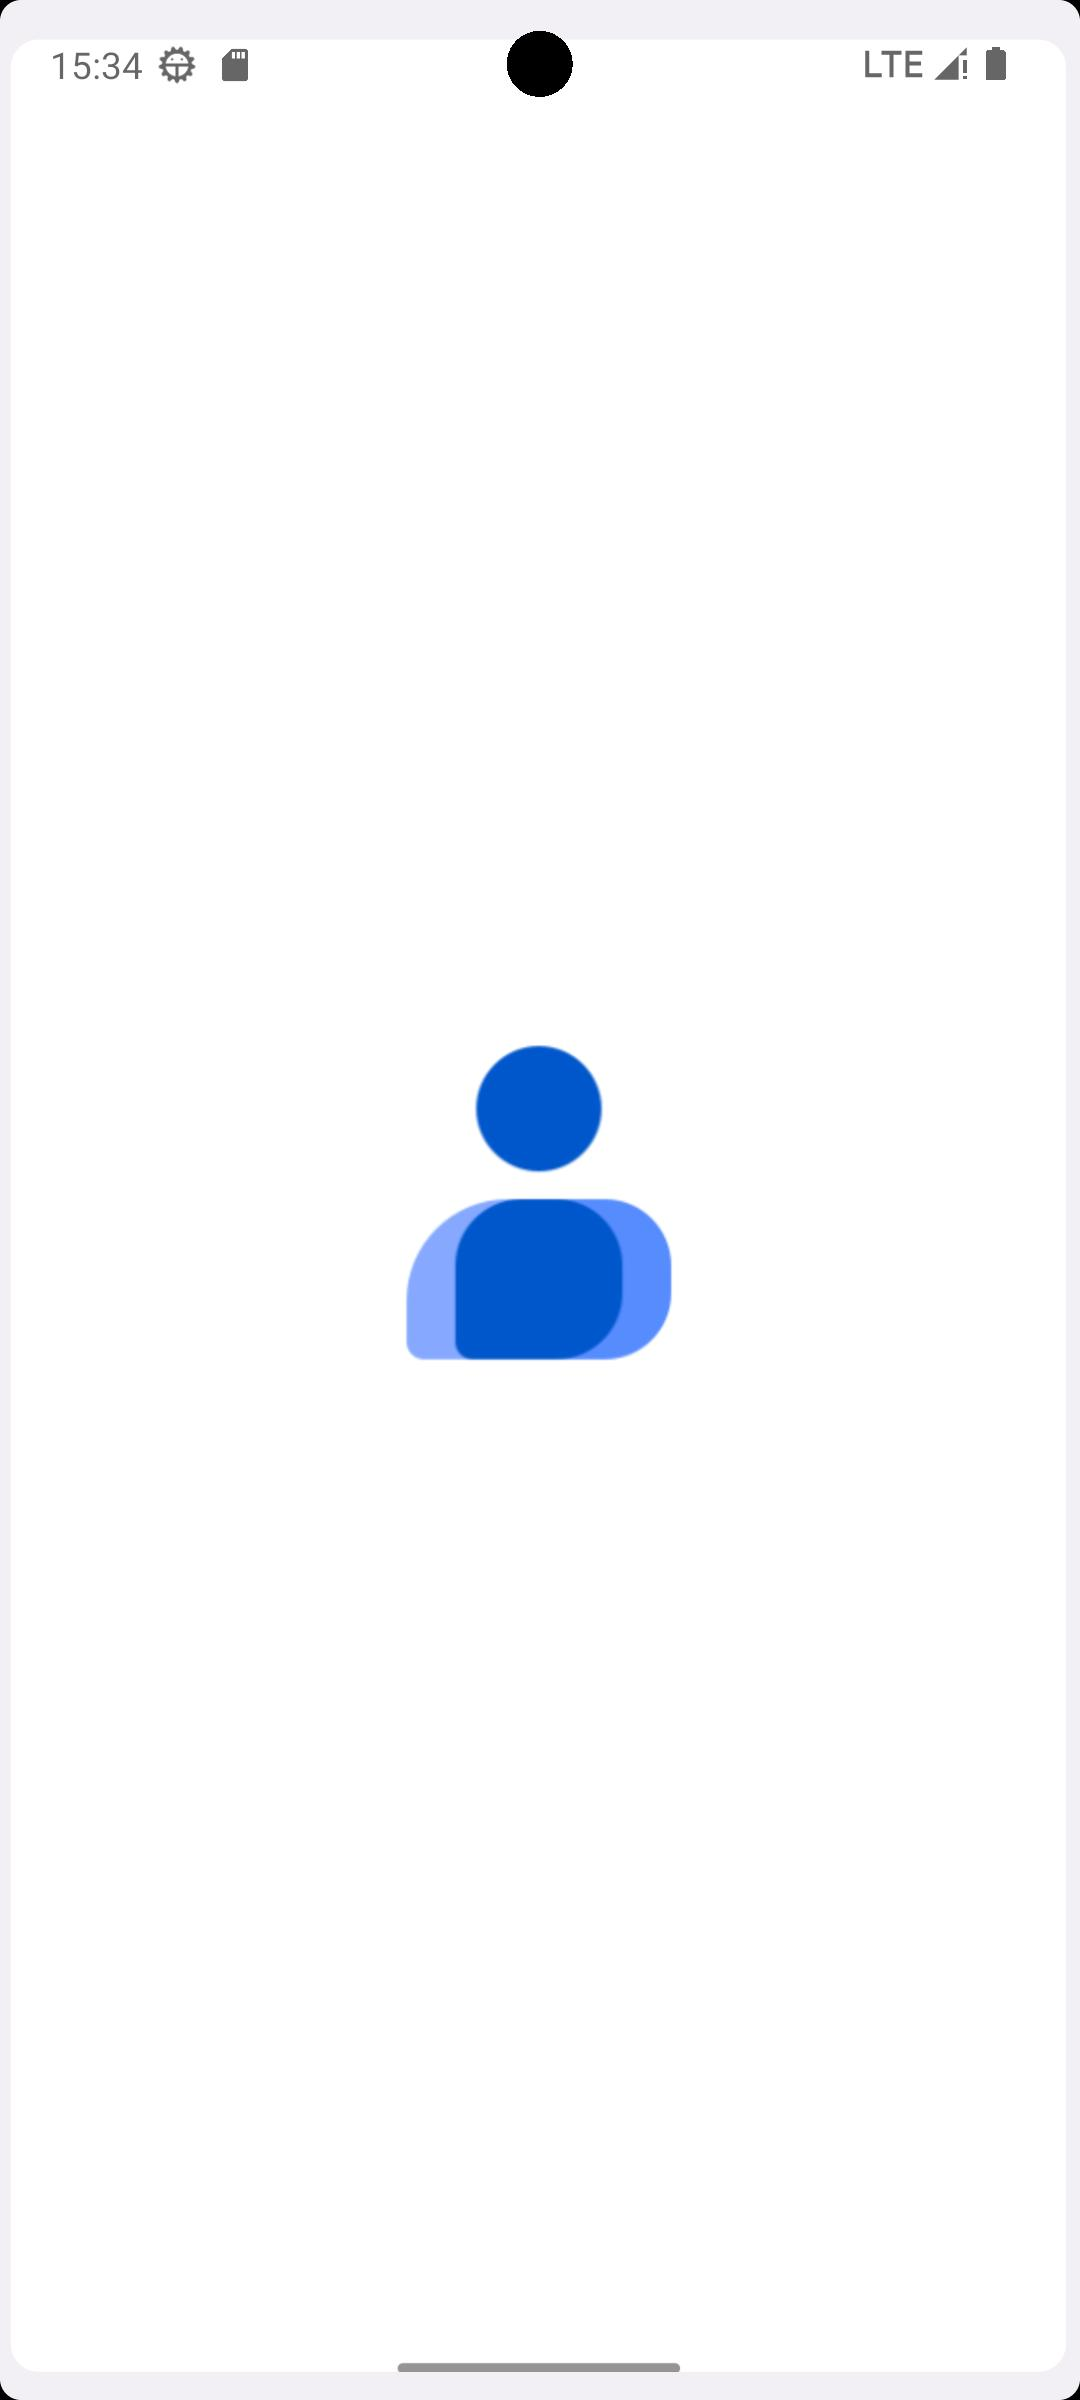}} &
        \parbox[t]{\linewidth}{
            \vspace{-3.5em}
            \textbf{\textit{[Step2]}}\\
            \textbf{Thought:} The app is loading; need to wait for initialization to access contact creation options. \\
            \textbf{Action:} \texttt{WAIT}
        } \\
        \hhline{-|-||-|-}  % 中间细线
        
        % Row 2: Step 3 & 4
        \raisebox{-0.5\height}{\includegraphics[width=\linewidth]{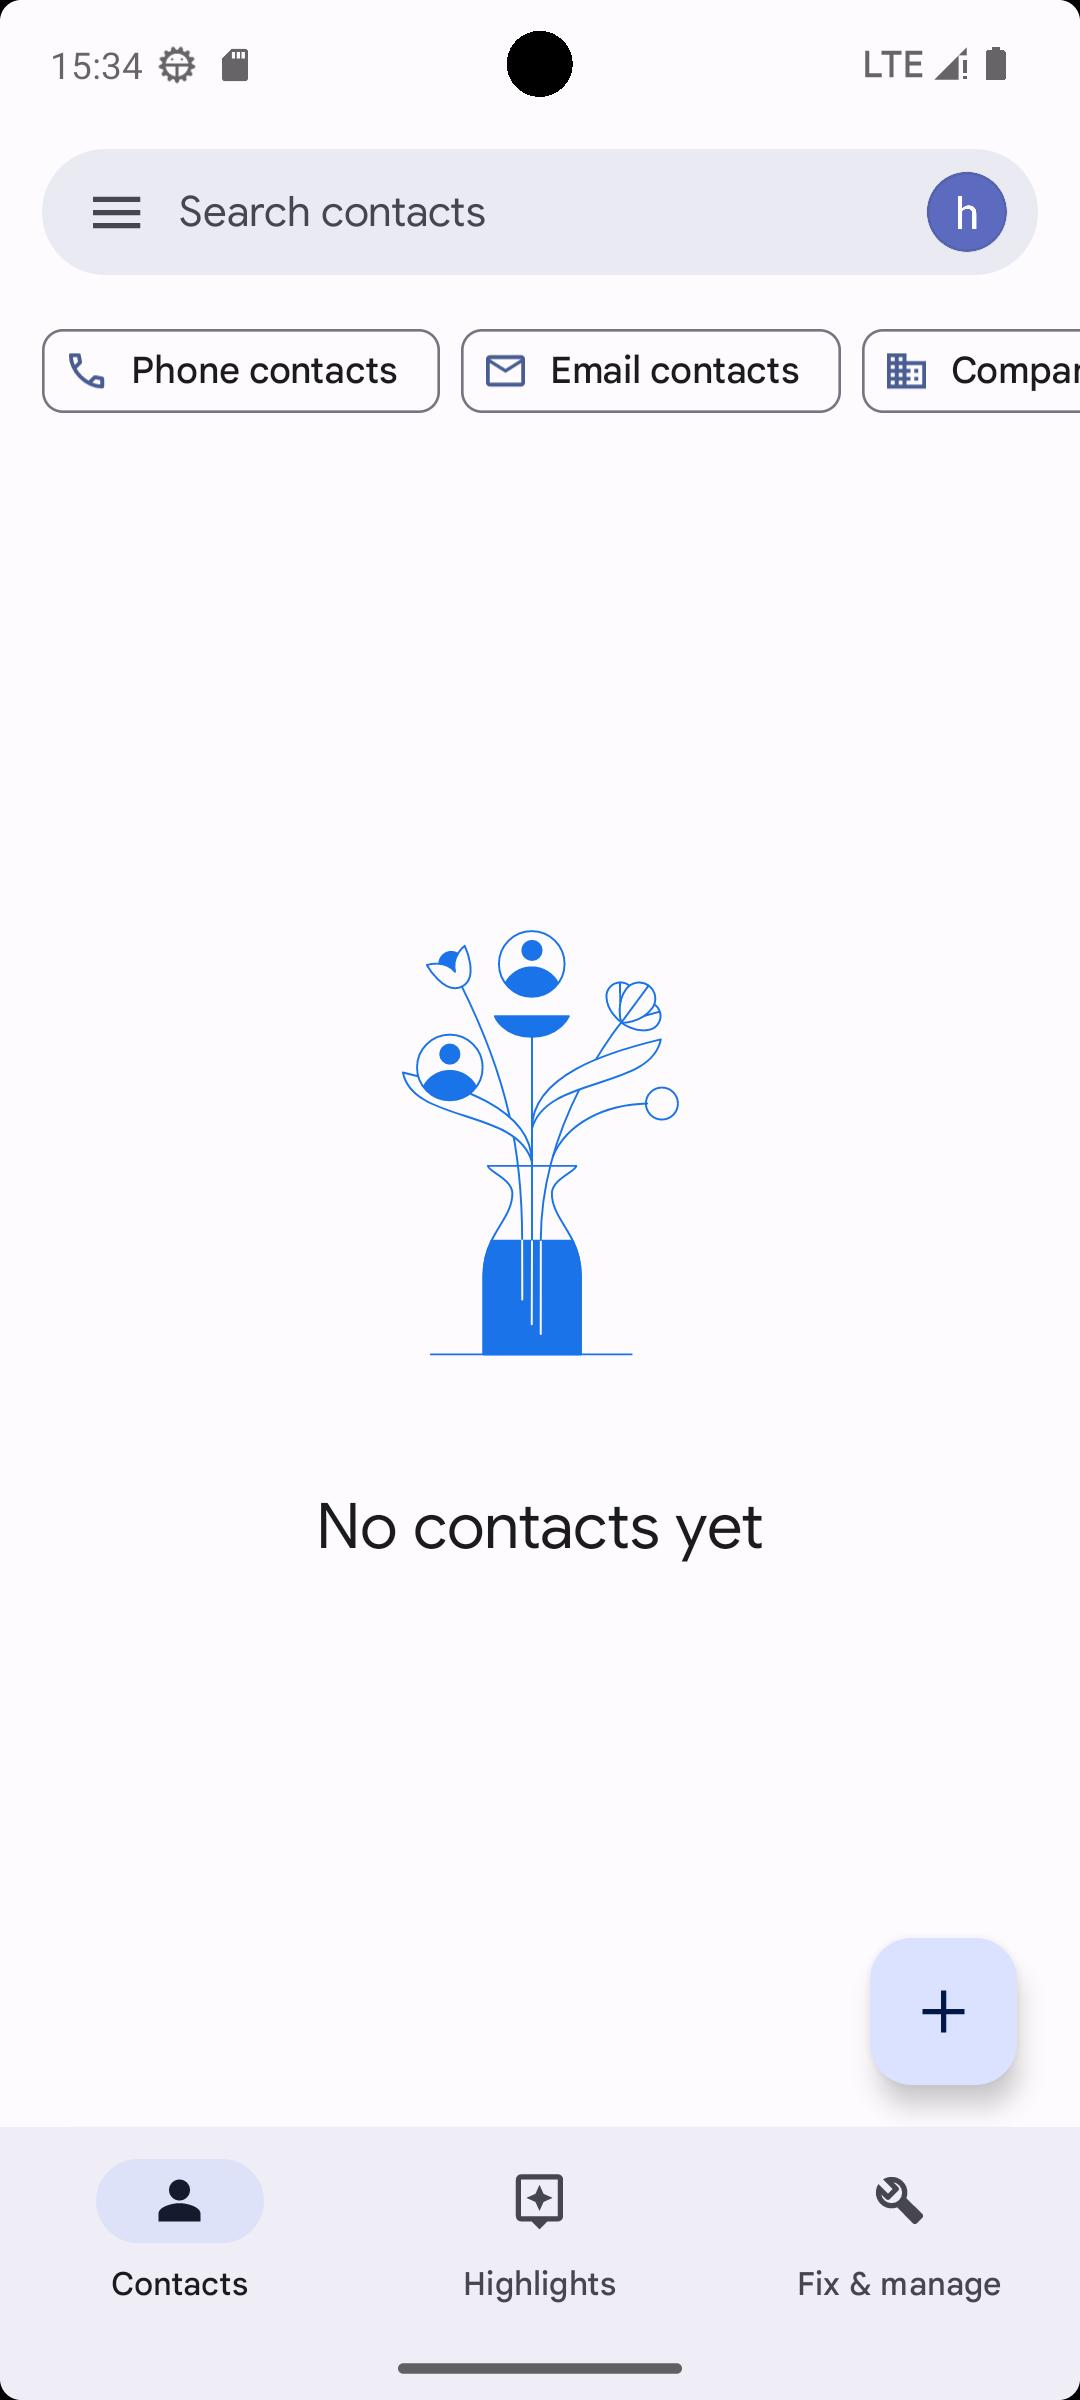}} &
        \parbox[t]{\linewidth}{
            \vspace{-3.5em}
            \textbf{\textit{[Step3]}}\\
            \textbf{Thought:} To create a new contact, I need to click the plus button to add new entries. \\
            \textbf{Action:} \texttt{pyautogui.click\\
            (x=0.871, y=0.827)}
        } &
        \raisebox{-0.5\height}{\includegraphics[width=\linewidth]{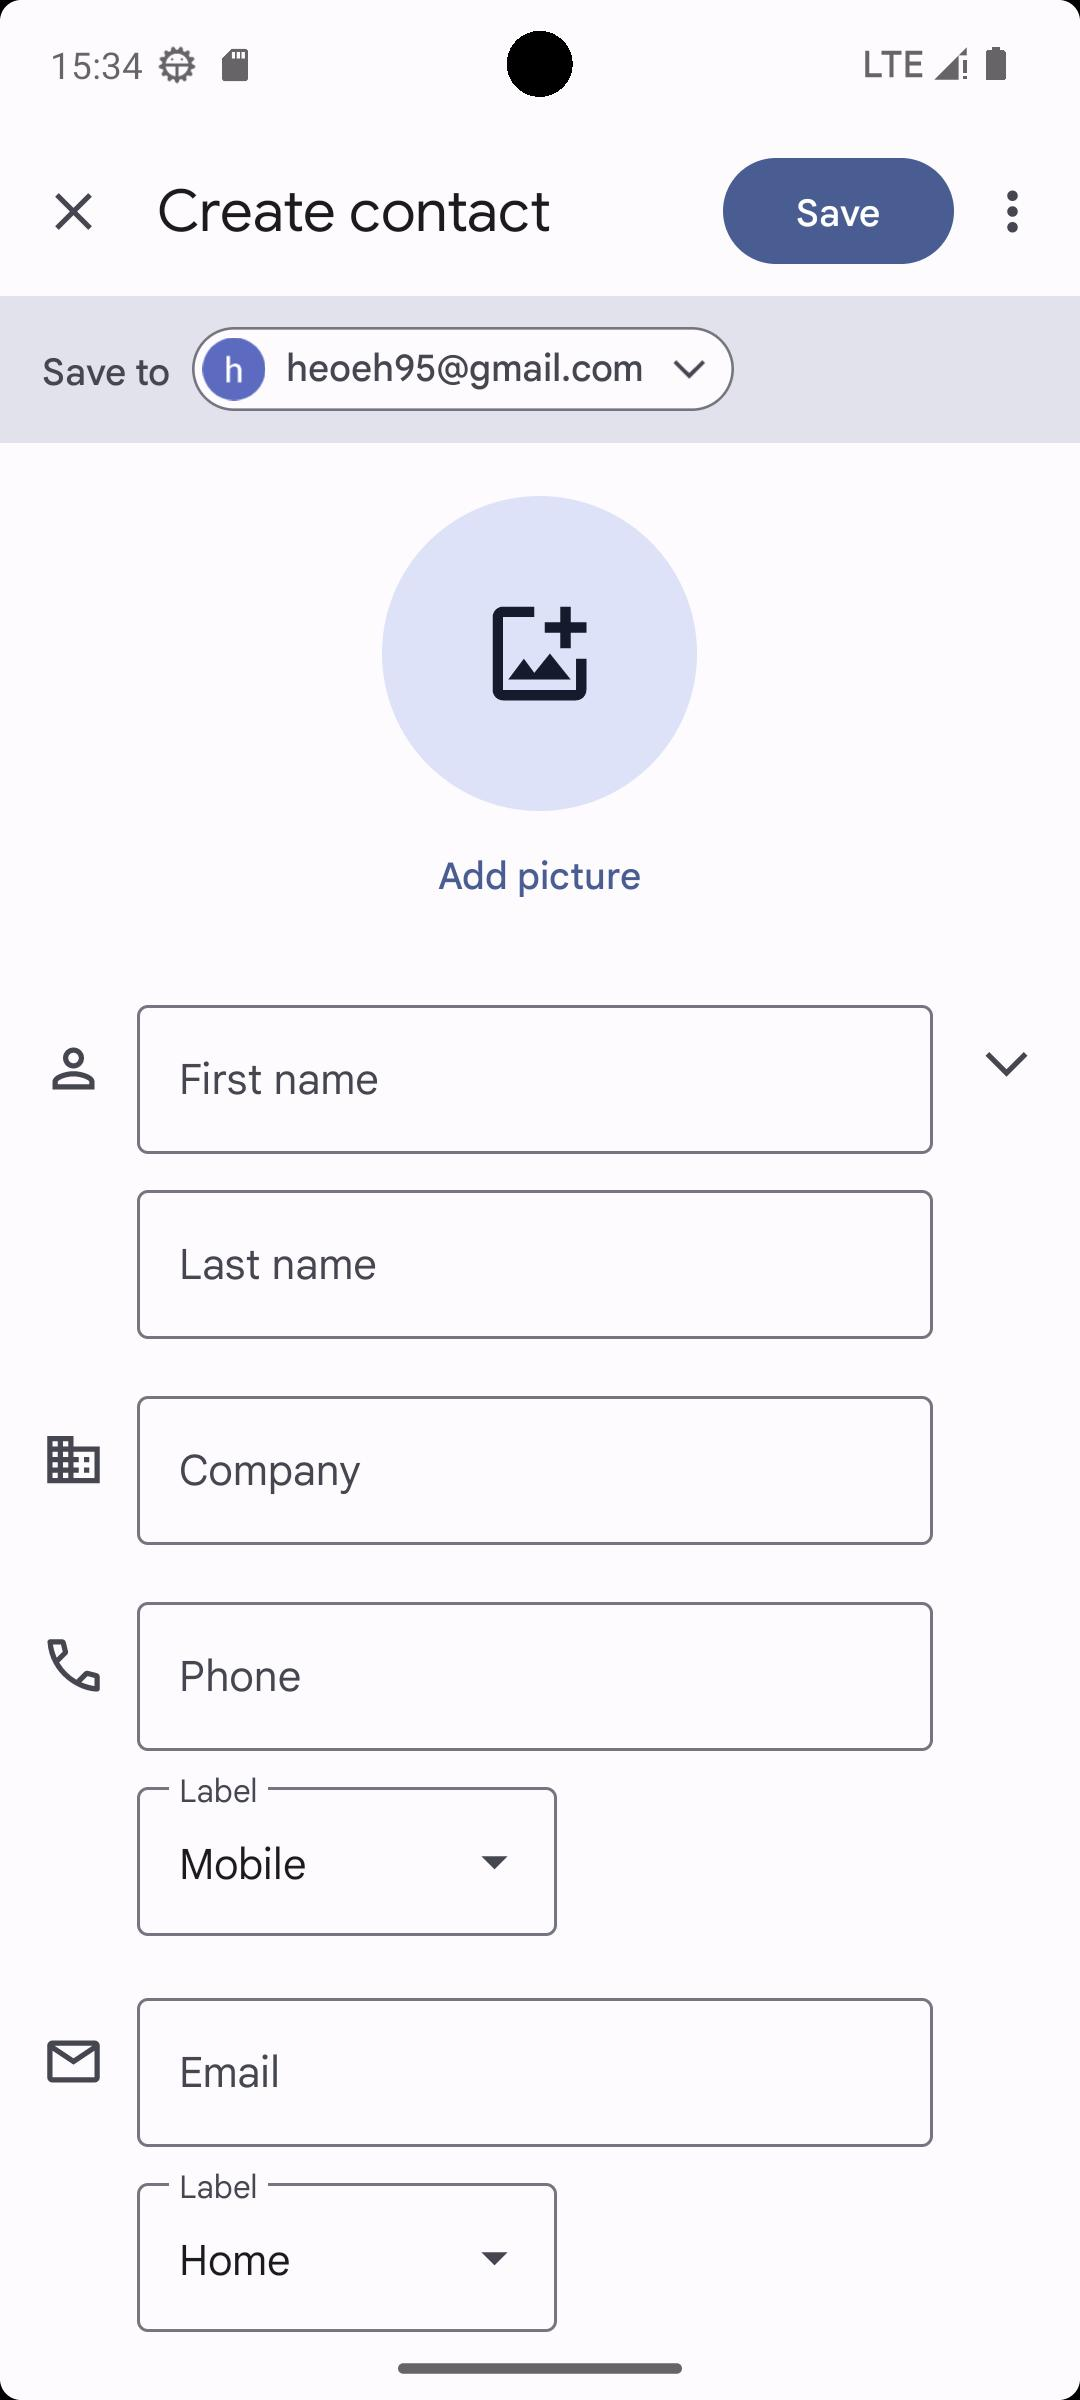}} &
        \parbox[t]{\linewidth}{
            \vspace{-3.5em}
            \textbf{\textit{[Step4]}}\\
            \textbf{Thought:} Activate phone number field to proceed with contact creation. \\
            \textbf{Action:} \texttt{pyautogui.click\\
            (x=0.332, y=0.706)}
        } \\
        \hhline{-|-||-|-}
        
        % Row 3: Step 5 & 6
        \raisebox{-0.5\height}{\includegraphics[width=\linewidth]{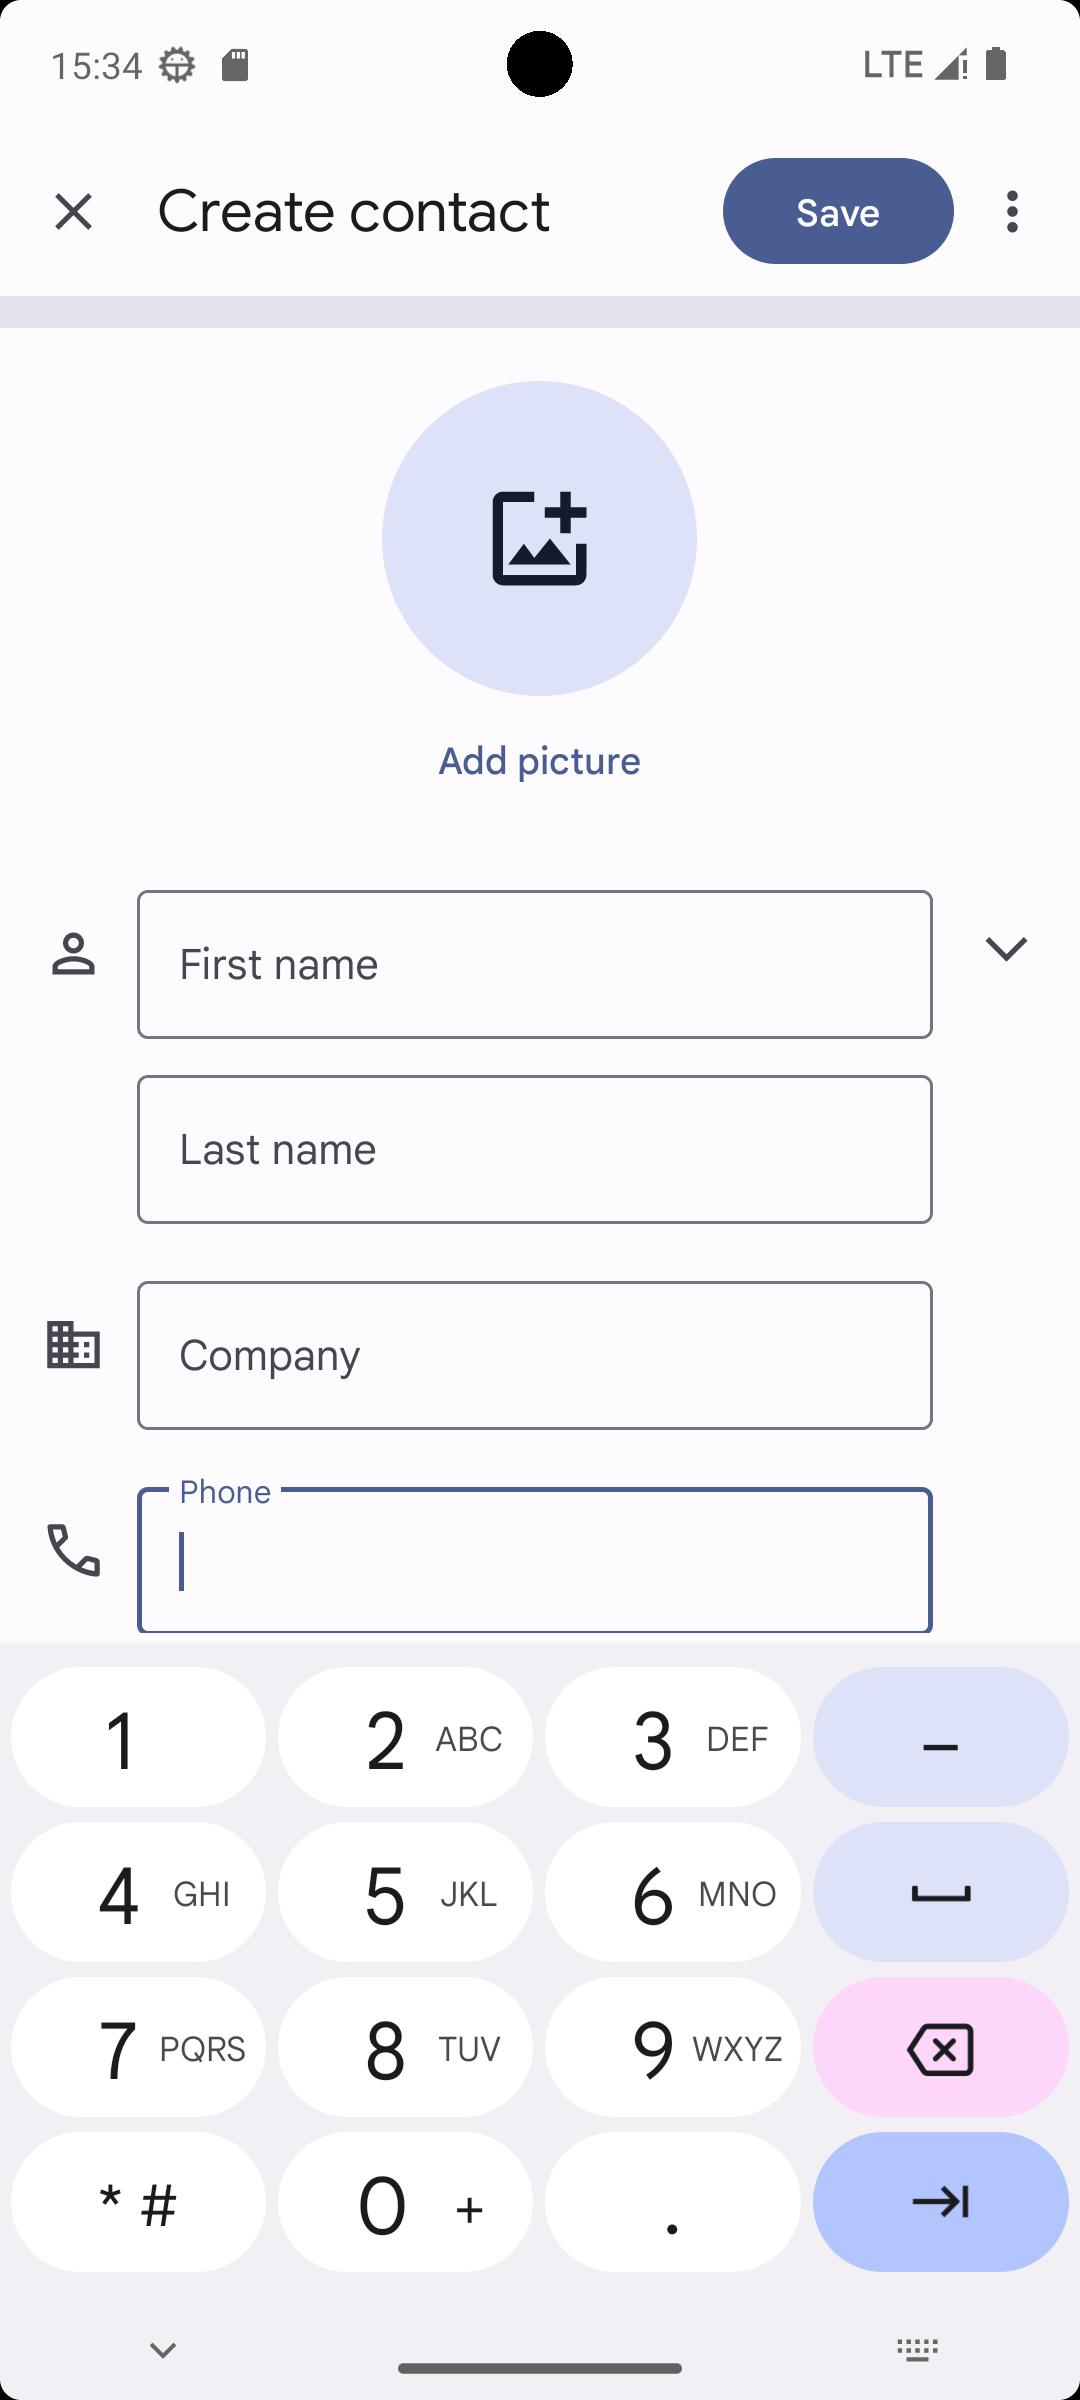}} &
        \parbox[t]{\linewidth}{
            \vspace{-3.5em}
            \textbf{\textit{[Step5]}}\\
            \textbf{Thought:} Entering phone number to create \\
            contact. \\
            \textbf{Action:} \texttt{pyautogui.write\\
            (message='+13920741751')}
        } &
        \raisebox{-0.5\height}{\includegraphics[width=\linewidth]{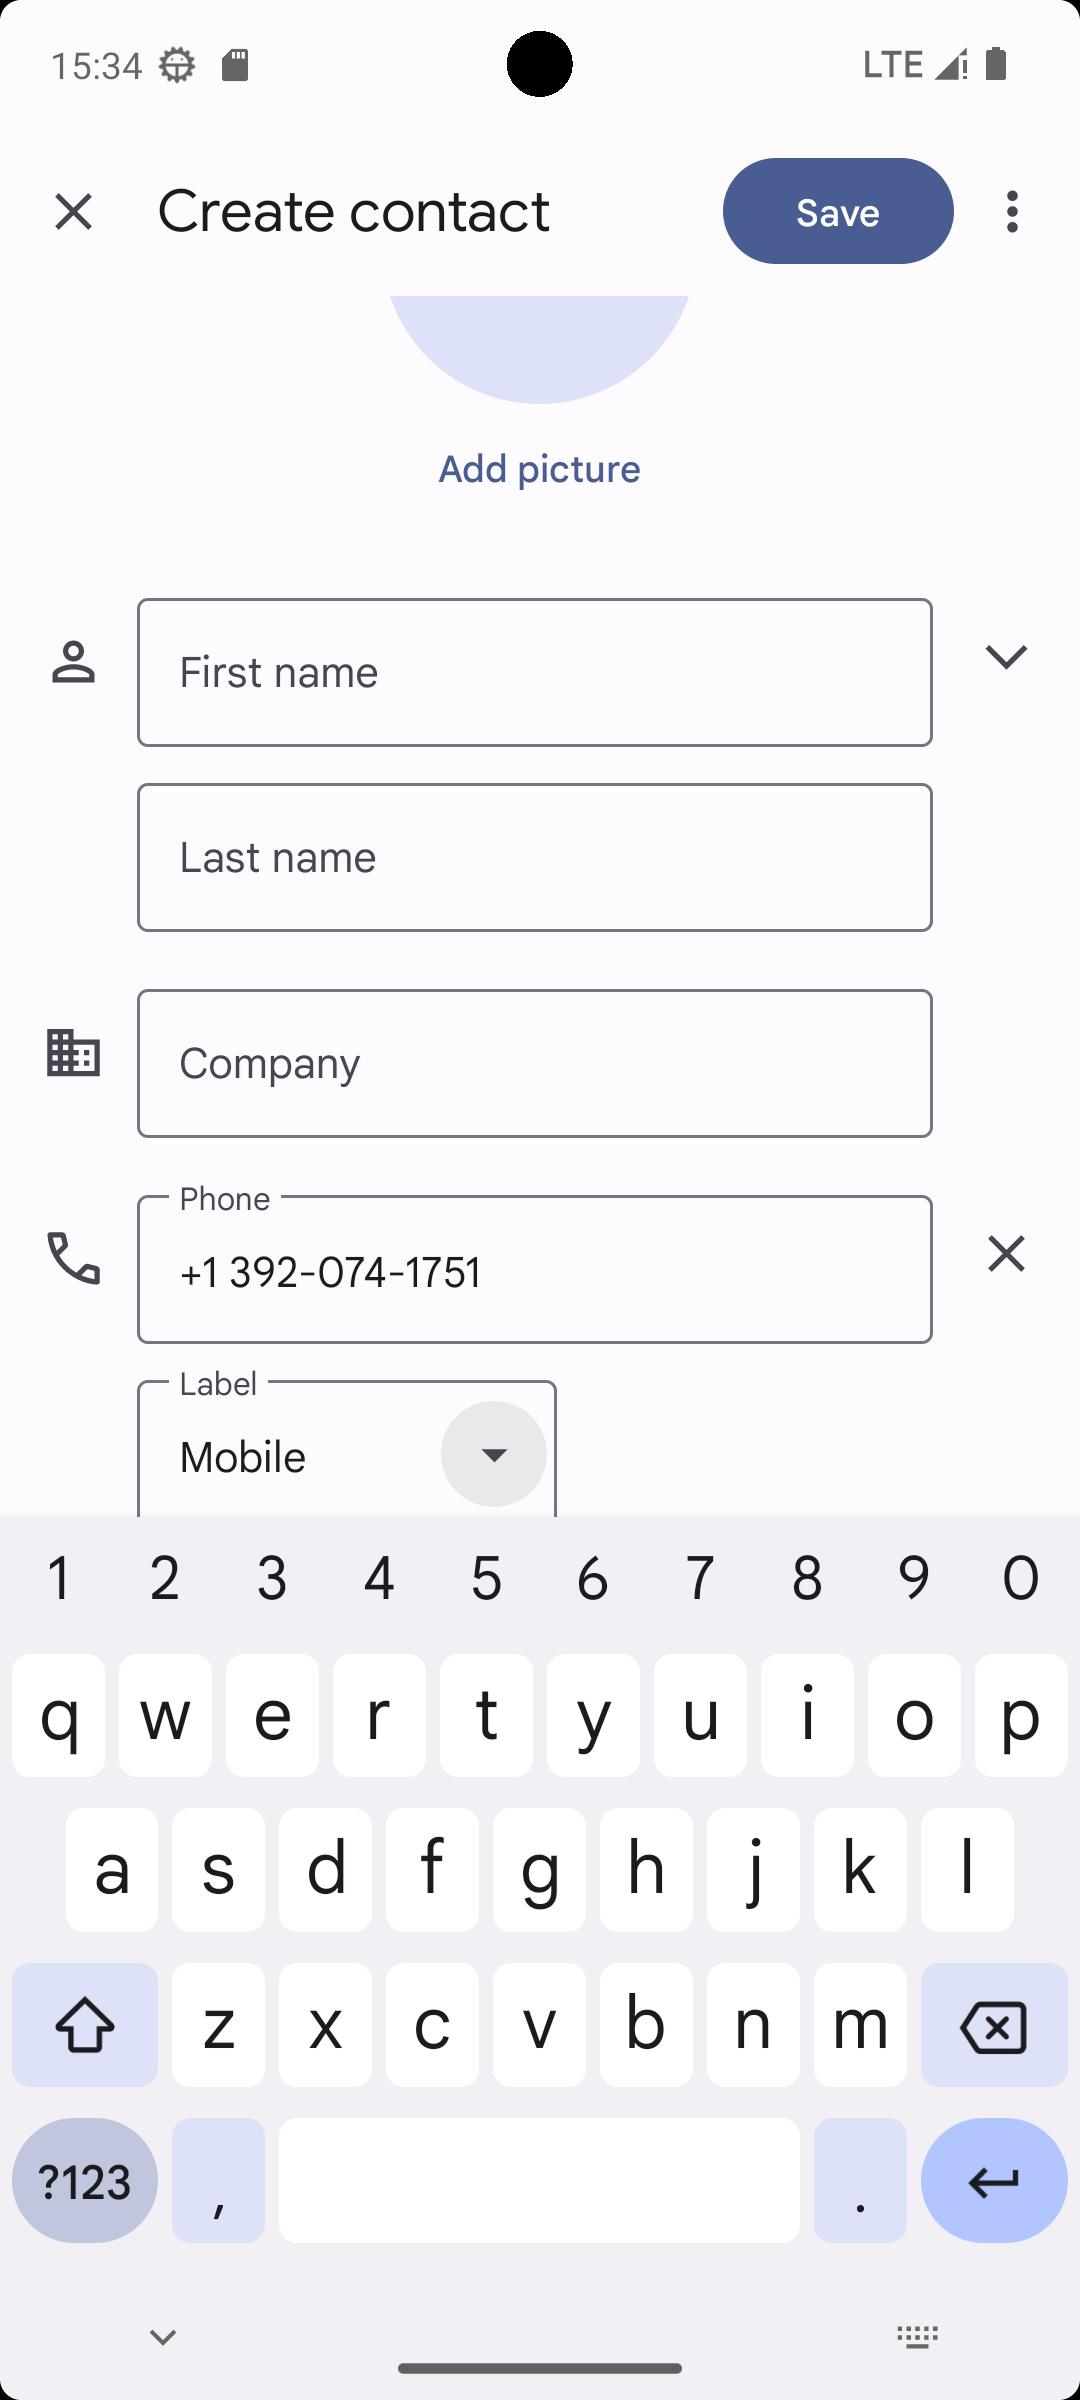}} &
        \parbox[t]{\linewidth}{
            \vspace{-3.5em}
            \textbf{\textit{[Step6]}}\\
            \textbf{Thought:} Completing contact info by filling 'First name' field. \\
            \textbf{Action:} \texttt{pyautogui.click\\
            (x=0.381, y=0.288)}
        } \\
        \hhline{-|-||-|-}
        
        % Row 4: Step 7 & 8
        \raisebox{-0.5\height}{\includegraphics[width=\linewidth]{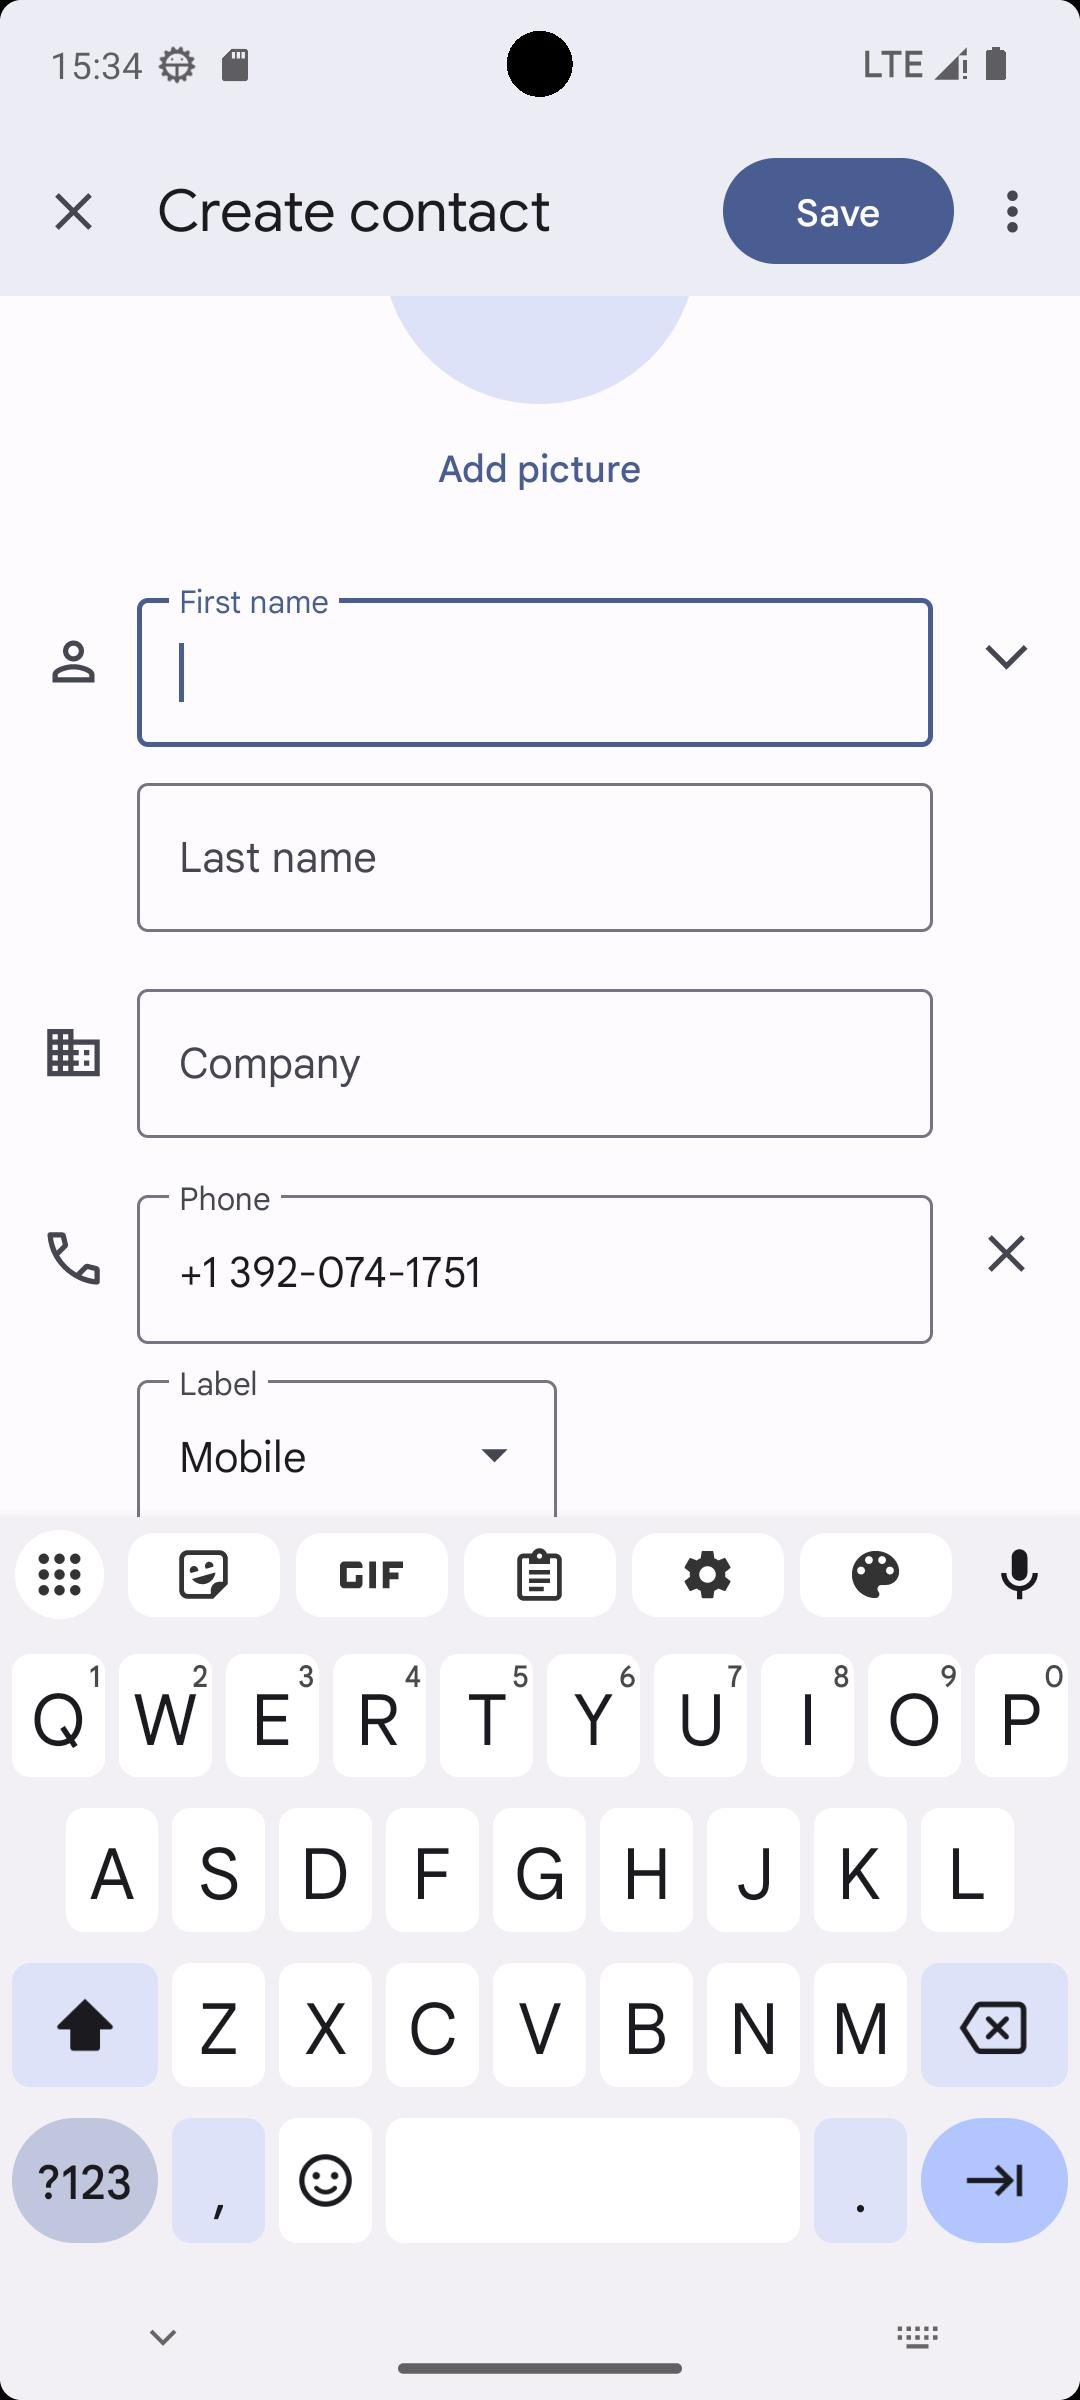}} &
        \parbox[t]{\linewidth}{
            \vspace{-3.5em}
            \textbf{\textit{[Step7]}}\\
            \textbf{Thought:} Filling in 'First name' field with 'Hugo' for contact creation. \\
            \textbf{Action:} \texttt{pyautogui.write\\
            (message='Hugo')}
        } &
        \raisebox{-0.5\height}{\includegraphics[width=\linewidth]{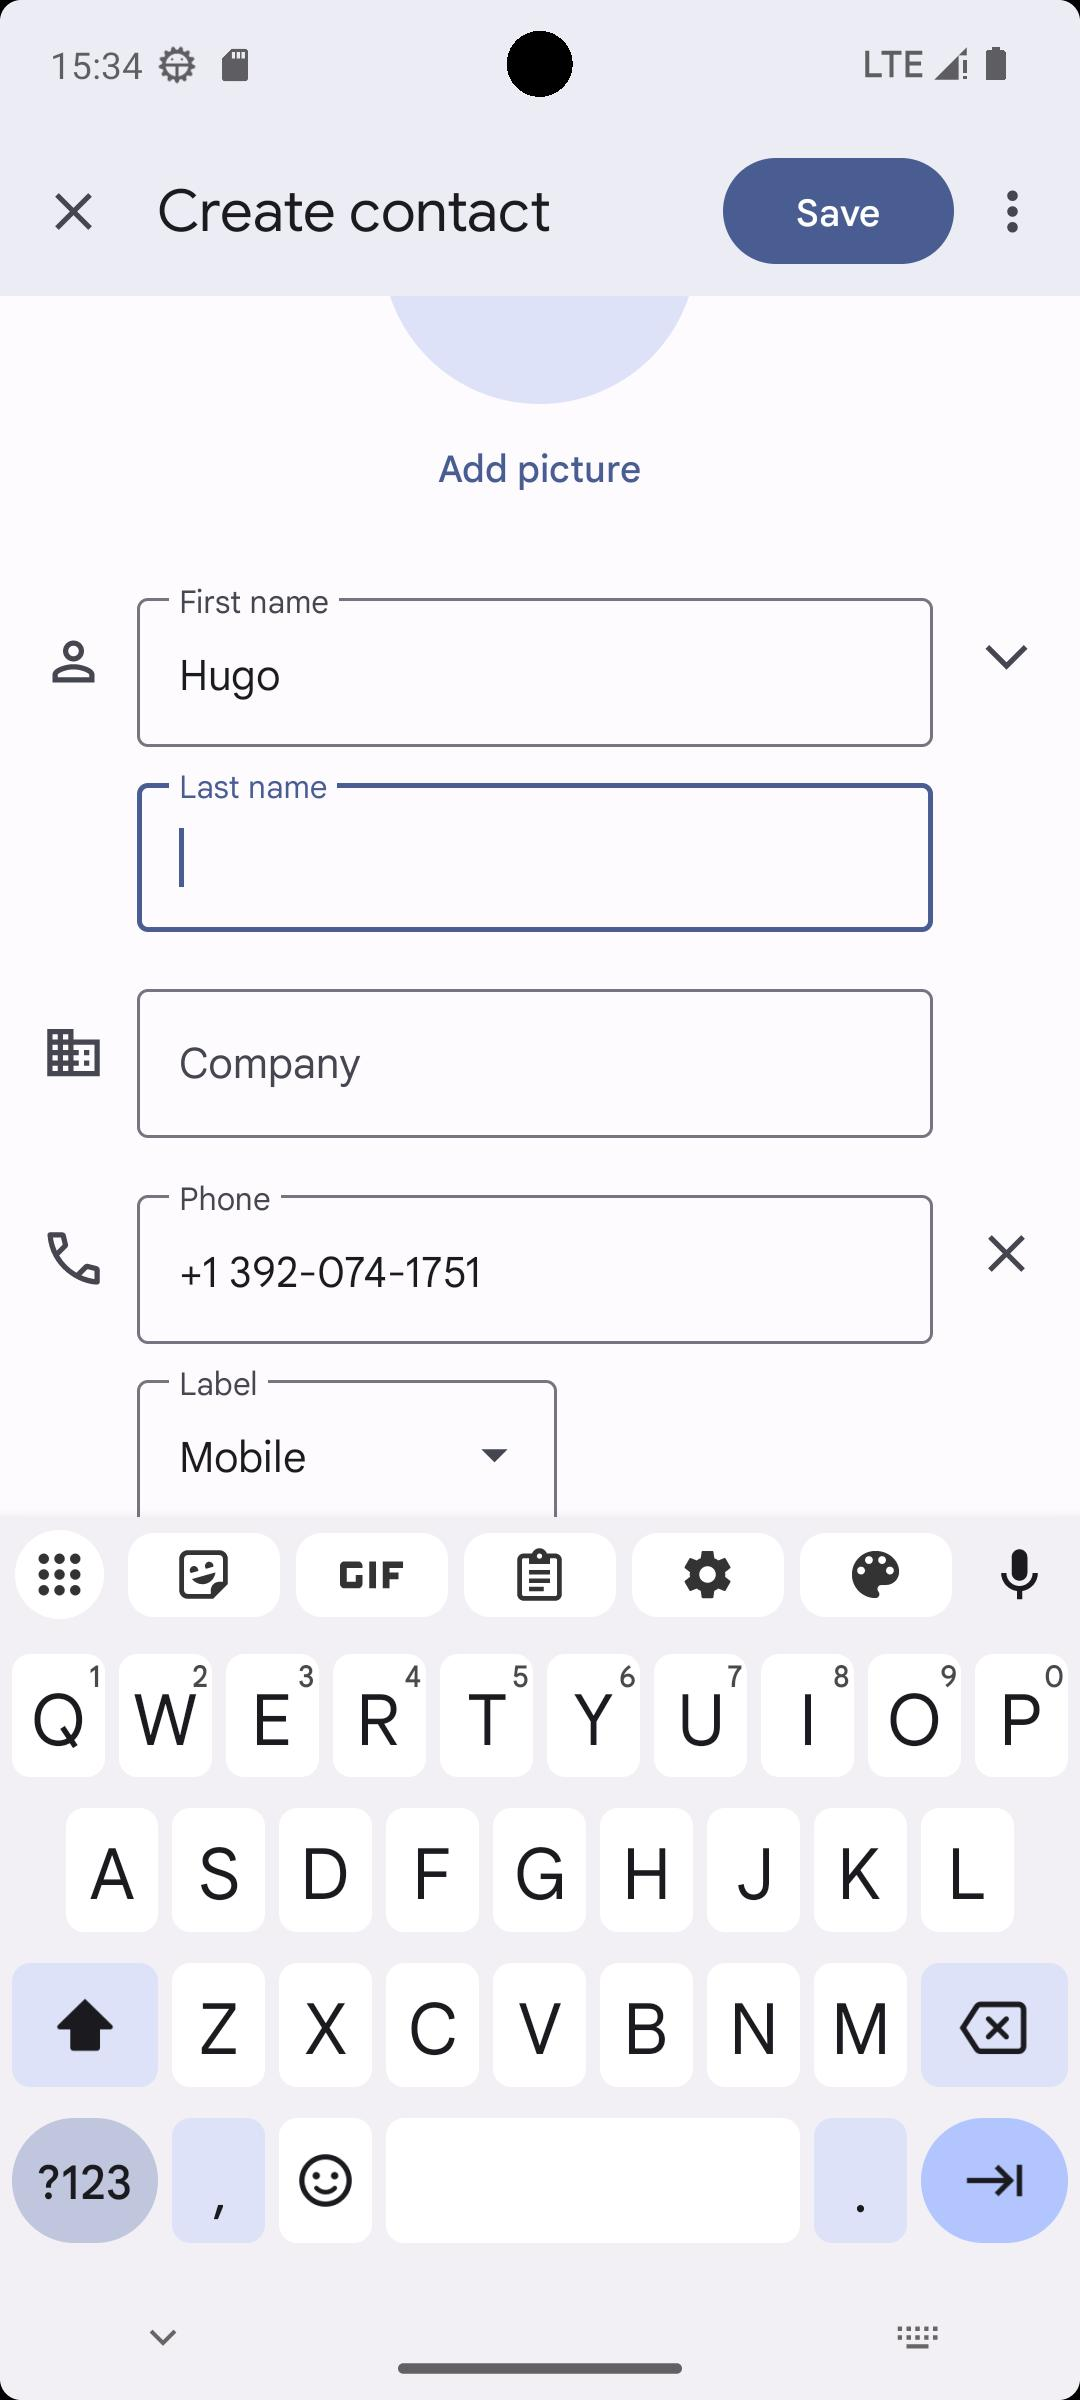}} &
        \parbox[t]{\linewidth}{
            \vspace{-3.5em}
            \textbf{\textit{[Step8]}}\\
            \textbf{Thought:} Entering last name 'Pereira' to complete contact details. \\
            \textbf{Action:} \texttt{pyautogui.write\\
            (message='Pereira')}
        } \\
        \hhline{-|-||-|-}
        
        % Row 5: Step 9 & 10
        \raisebox{-0.5\height}{\includegraphics[width=\linewidth]{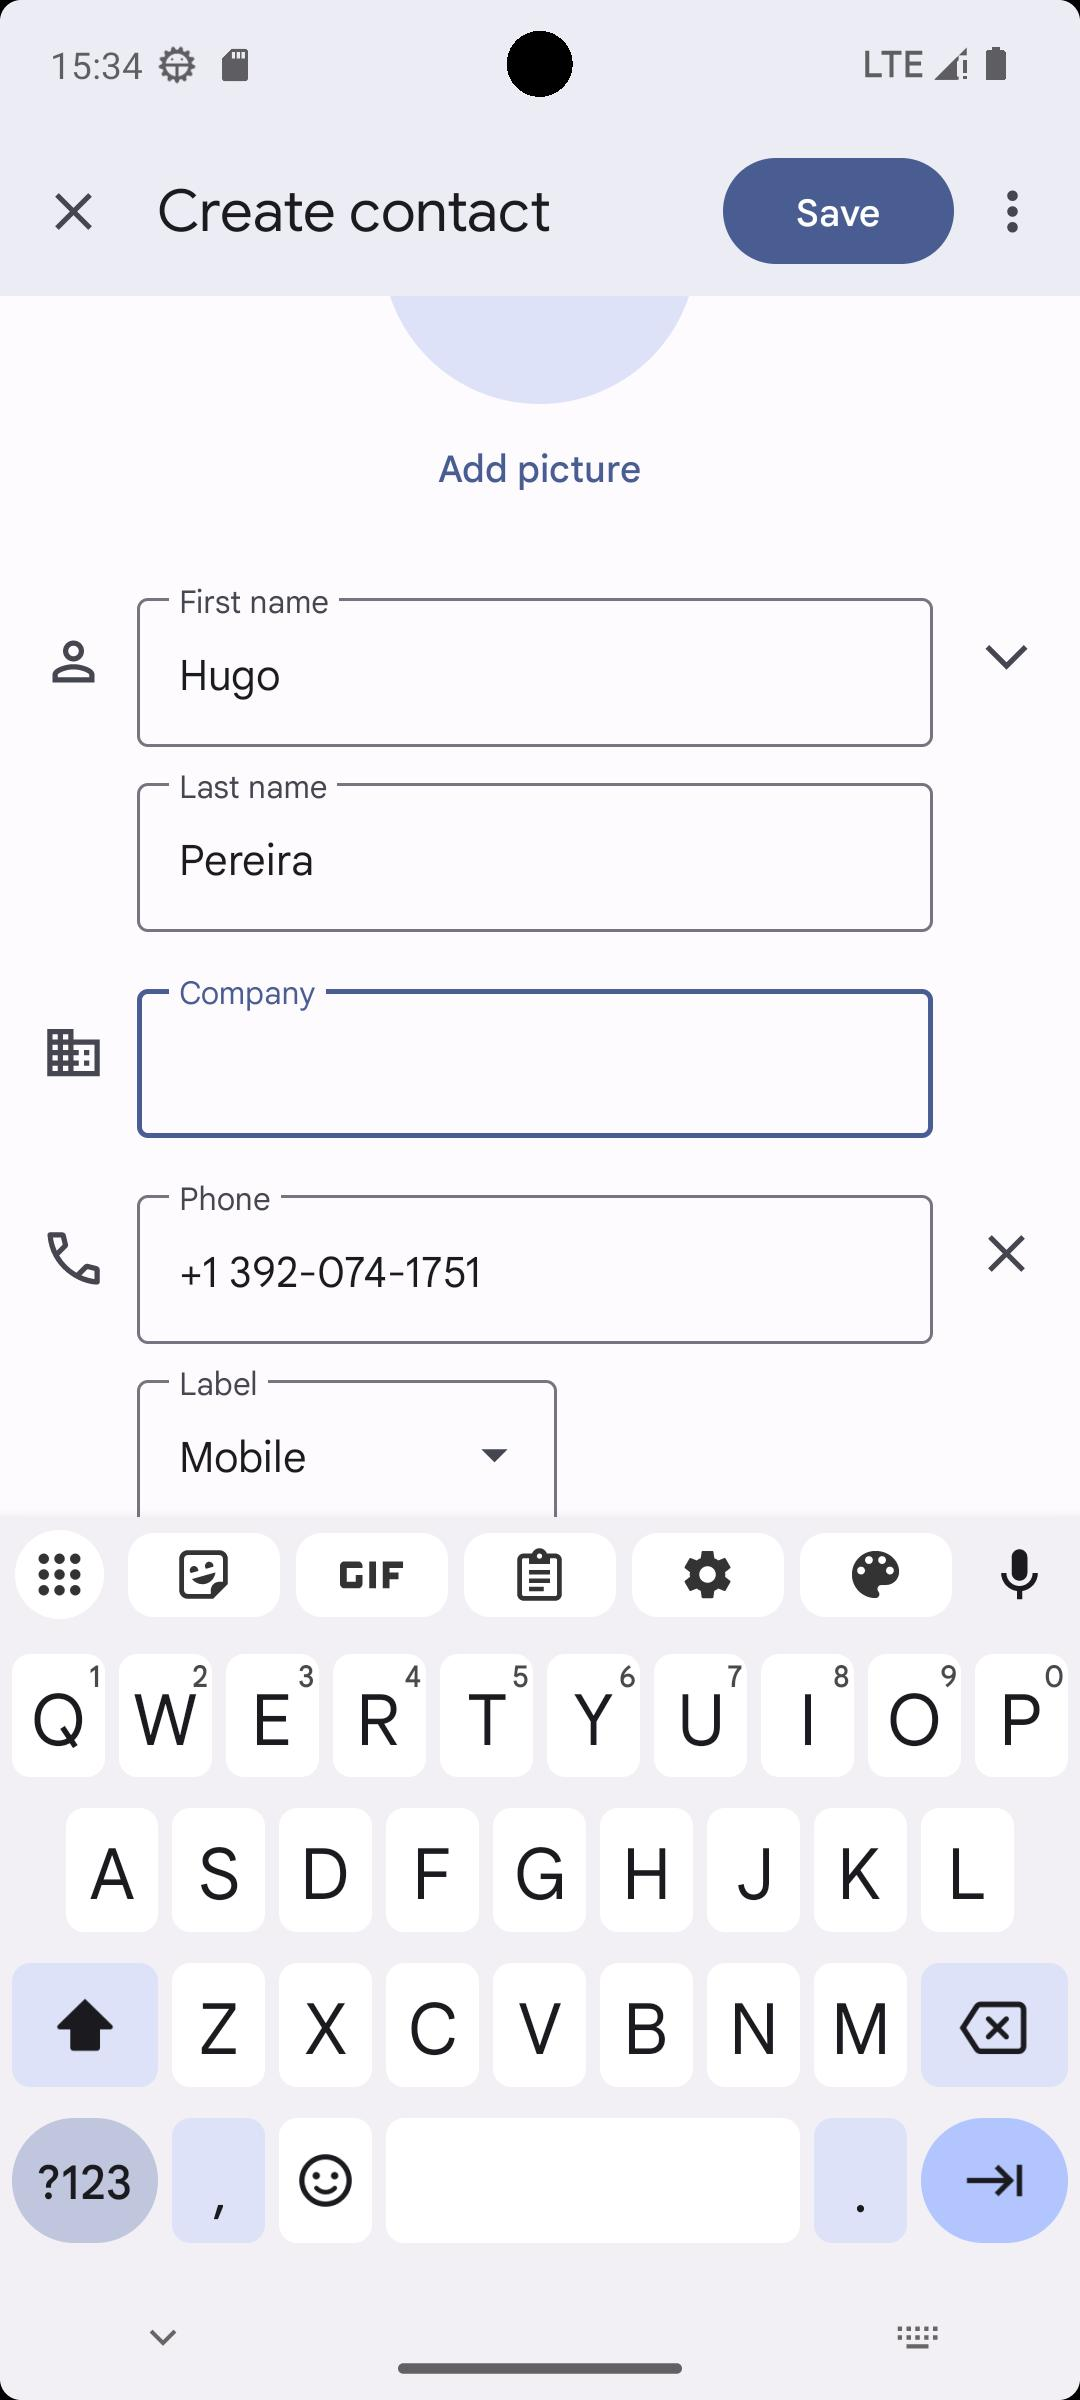}} &
        \parbox[t]{\linewidth}{
            \vspace{-3.5em}
            \textbf{\textit{[Step9]}}\\
            \textbf{Thought:} Contact details are complete; ready to save. \\
            \textbf{Action:} \texttt{pyautogui.click\\
            (x=0.775, y=0.098)}
        } &
        \raisebox{-0.5\height}{\includegraphics[width=\linewidth]{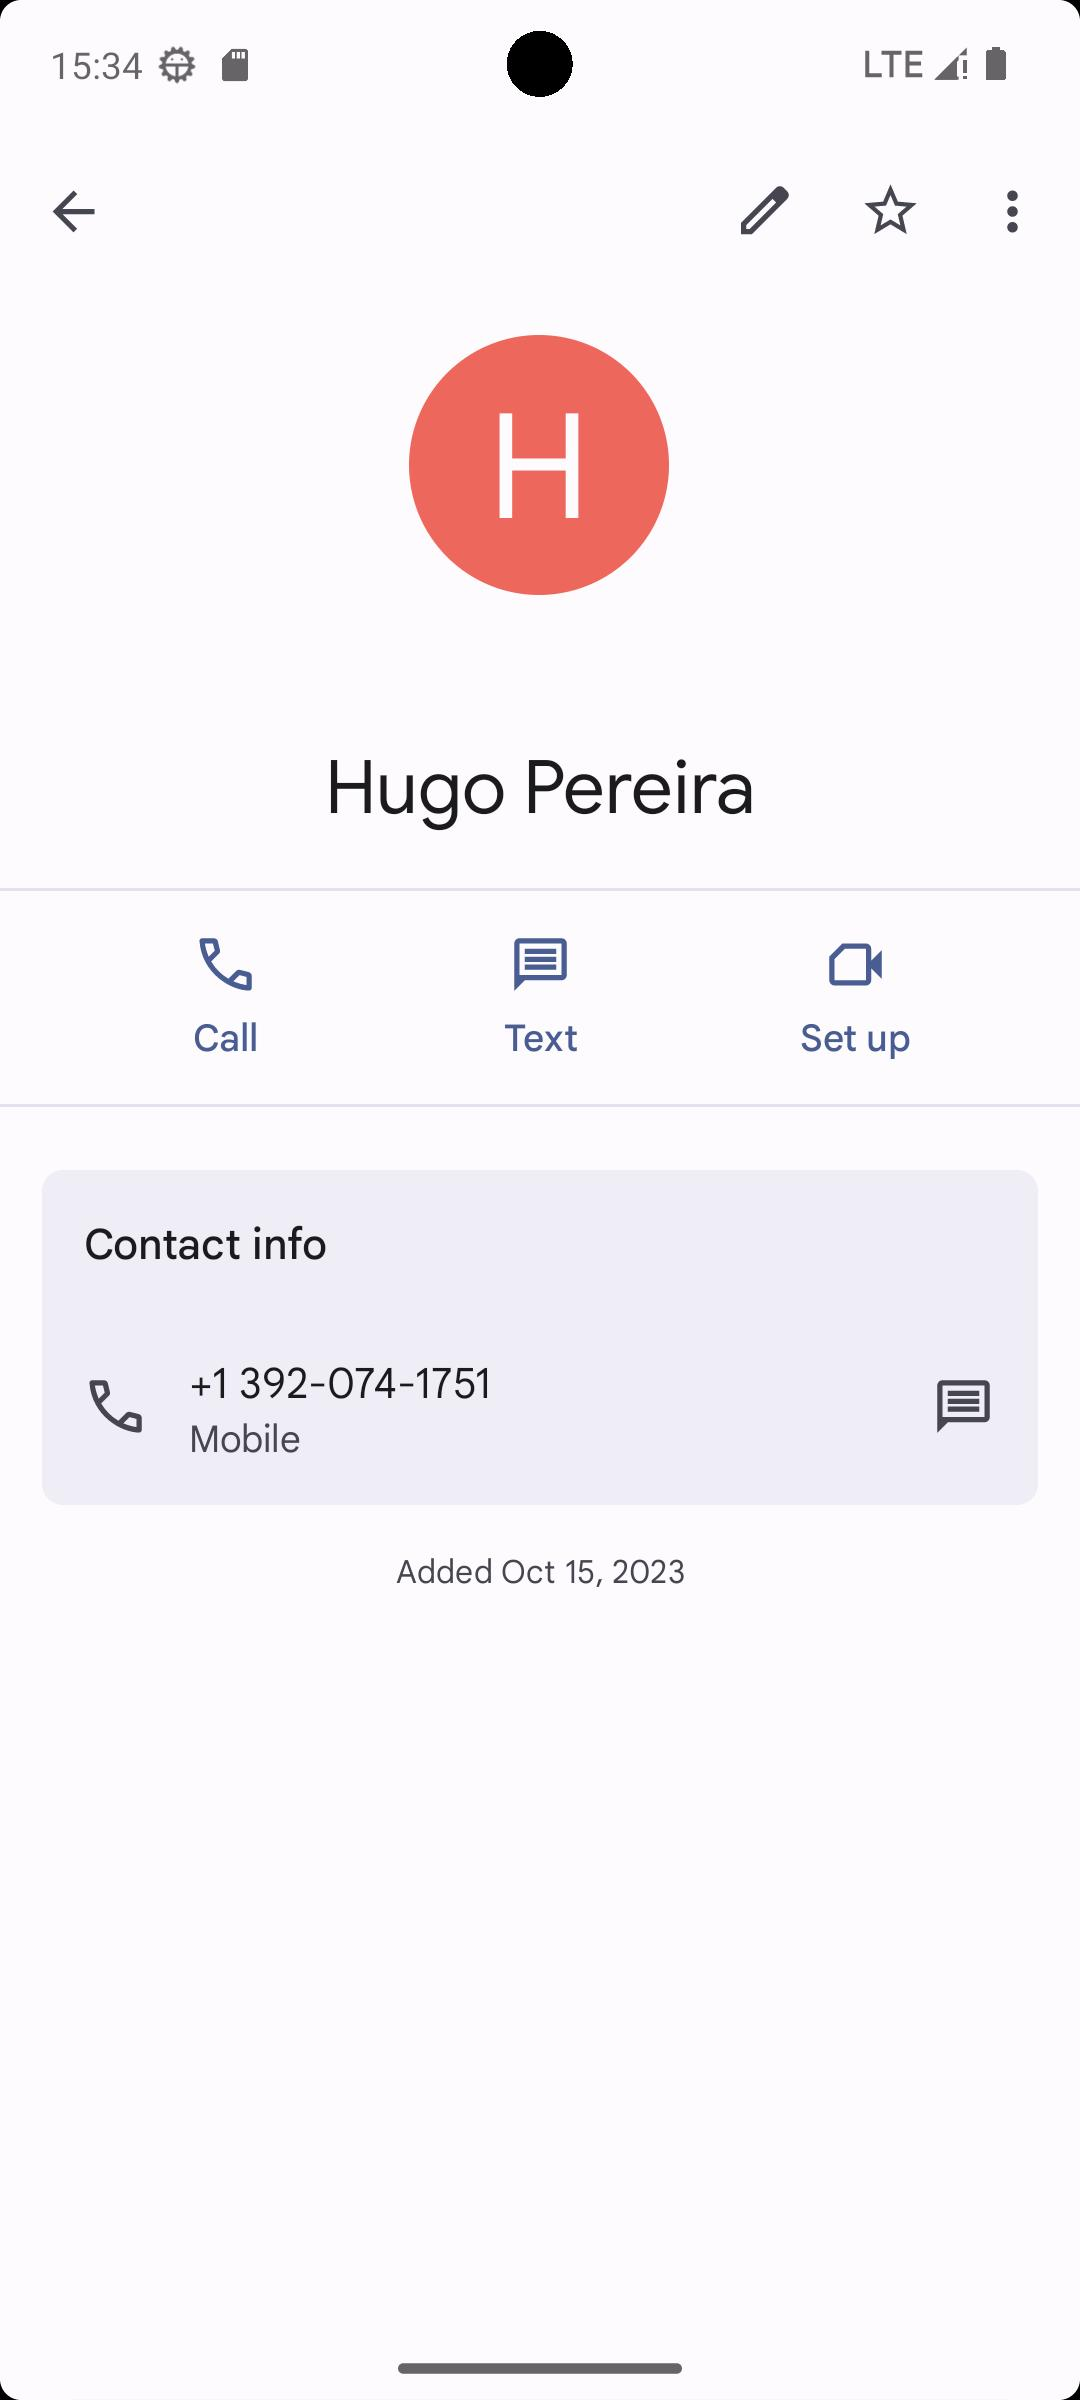}} &
        \parbox[t]{\linewidth}{
            \vspace{-3.5em}
            \textbf{\textit{[Step10]}}\\
            \textbf{Thought:} Contact successfully created for Hugo Pereira. \\
            \textbf{Action:} \texttt{mobile.terminate\\
            (status='success')}
        } \\
        % --- Bottom: 细横线 ---
        \hhline{====}
    \end{tabular}
\end{table*}

\clearpage
